# Supplementary material for: Thermal and mechanical properties and the structural phase transition under pressure in $A$In$_2$As$_2$ ($A$ = Ca, Sr, Ba)
Source: arXiv:2407.03290 source file (2024-07-03)
Supplement: Supplementary file 1 [file Supplemental.pdf]

# Thermal and mechanical properties and the structural phase transition under pressure in $A\mathrm{In_2As_2}$ ($A$=Ca, Sr, Ba)

Wen-Ti Guo,[1,2] Zhigao Huang,[1,2] and Jian-Min Zhang[1,2,*]

[1]*Fujian Provincial Key Laboratory of Quantum Manipulation and New Energy Materials, College of Physics and Energy, Fujian Normal University, Fuzhou 350117, China*
[2]*Fujian Provincial Collaborative Innovation Center for Advanced High-Field Superconducting Materials and Engineering, Fuzhou, 350117, China*

## I. ADDITIONAL FIGURES

### A. Mechanical Properties

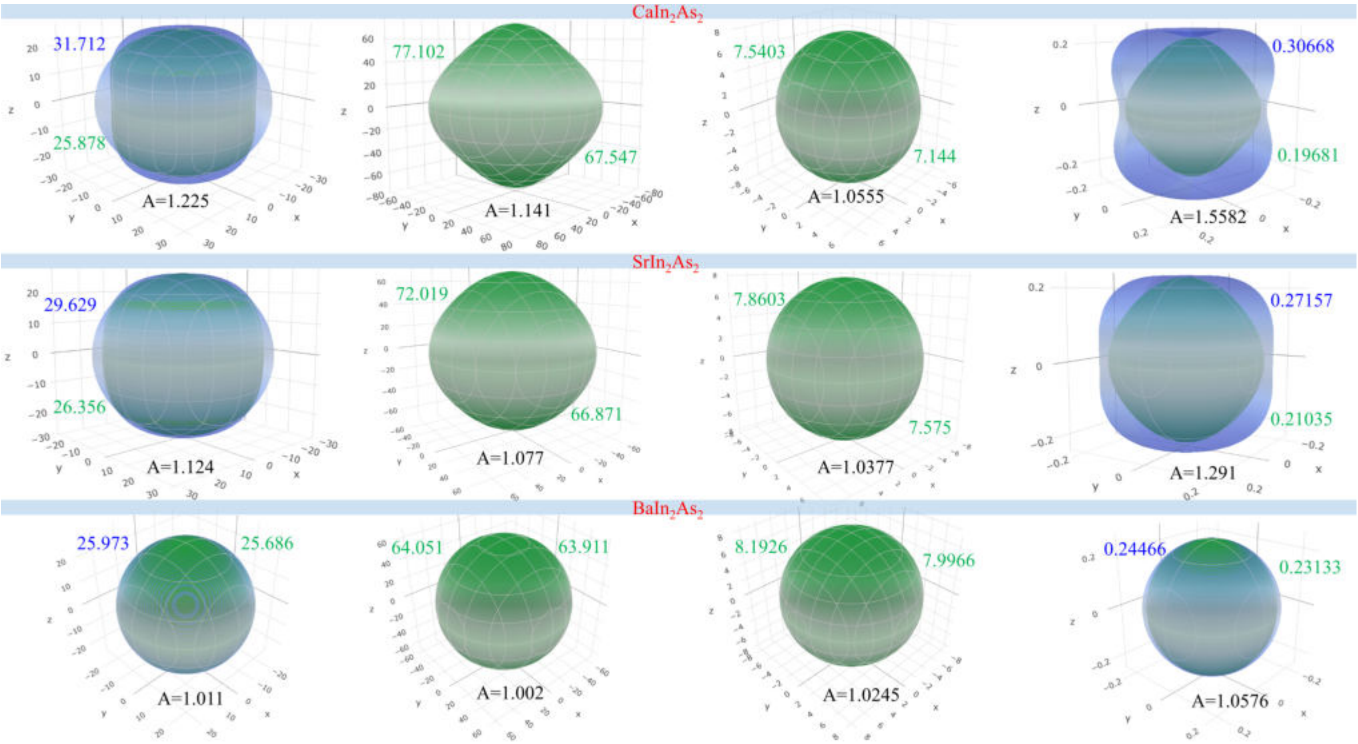


FIG. S1. The 3D form elastic modulus parameters of hexagonal ($P6_3/mmc$) AEIn$_2$As$_2$ without pressure include shear modulus $G$, Young's modulus $Y$, linear compression ($LC$), and Poisson's ratio ($v$). The blue and green surfaces indicate the maximum positive and minimum positive values of $G$, and the maximum positive value of $Y$ is indicated by the green surface. The positive values of $LC$ are represented in green surface, and those of negative $LC$ are represented in red surface. For $v$, the maximum (blue), minimum positive (green), and minimum negative (red) values.

* Corresponding authorjmzhang@fjnu.edu.cn

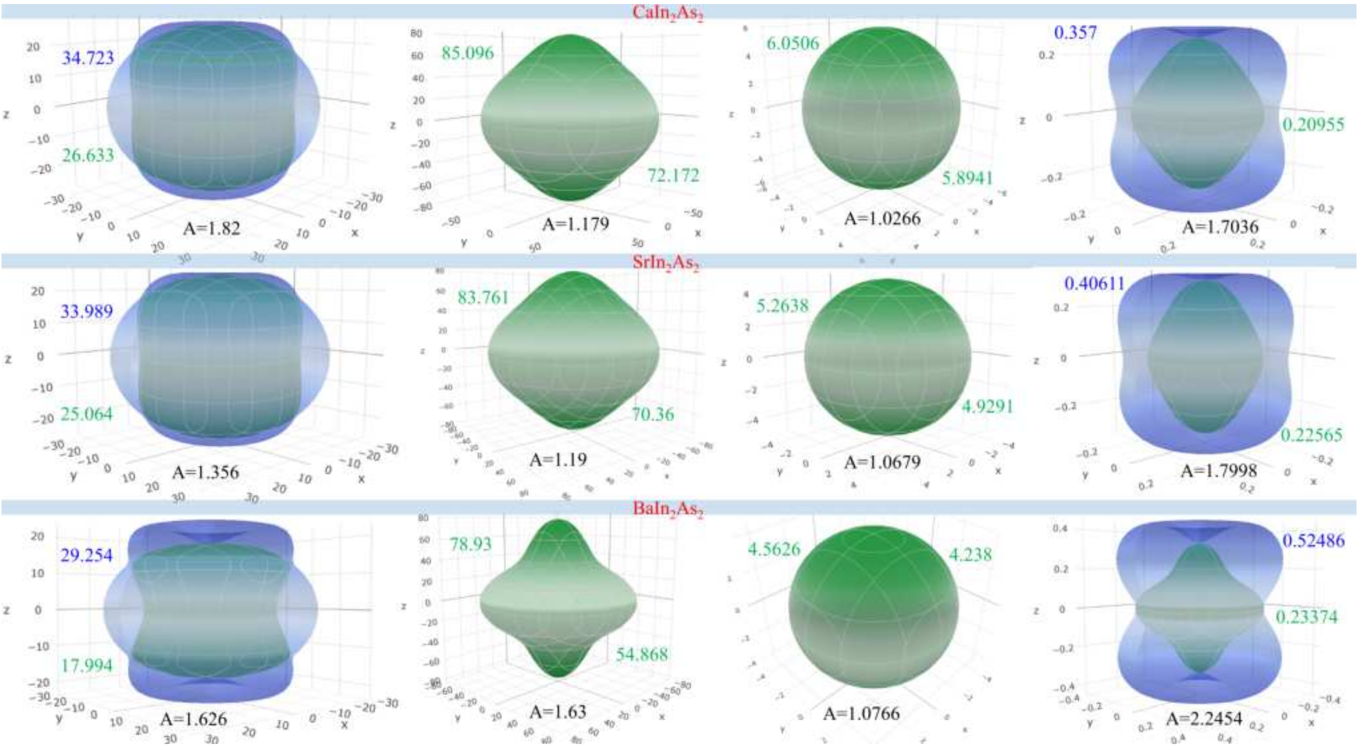


FIG. S2. The 3D form elastic modulus parameters of hexagonal ($P6_3/mmc$) $AEIn_2As_2$ induced zero band gap under pressure include shear modulus $G$, Young's modulus $Y$, linear compression ($LC$), and Poisson's ratio ($v$). The blue and green surfaces indicate the maximum positive and minimum positive values of $G$, and the maximum positive value of $Y$ is indicated by the green surface. The positive values of $LC$ are represented in green surface, and those of negative $LC$ are represented in red surface. For $v$, the maximum (blue), minimum positive (green), and minimum negative (red) values.

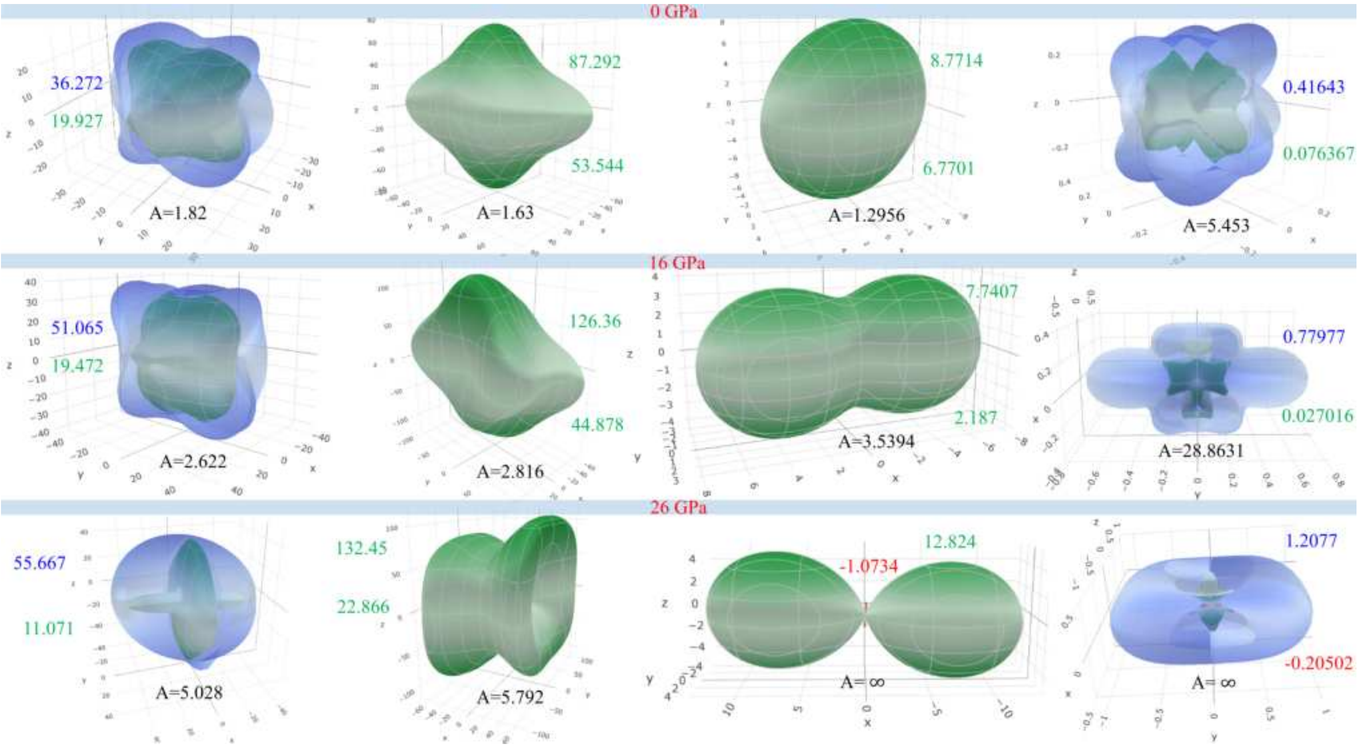


FIG. S3. The 3D form elastic modulus parameters of monoclinic $CaIn_2As_2$ under different pressures include shear modulus $G$, Young's modulus $Y$, linear compression ($LC$), and Poisson's ratio ($v$). The blue and green surfaces indicate the maximum positive and minimum positive values of $G$, and the maximum positive value of $Y$ is indicated by the green surface. The positive values of $LC$ are represented in green surface, and those of negative $LC$ are represented in red surface. For $v$, the maximum (blue), minimum positive (green), and minimum negative (red) values.

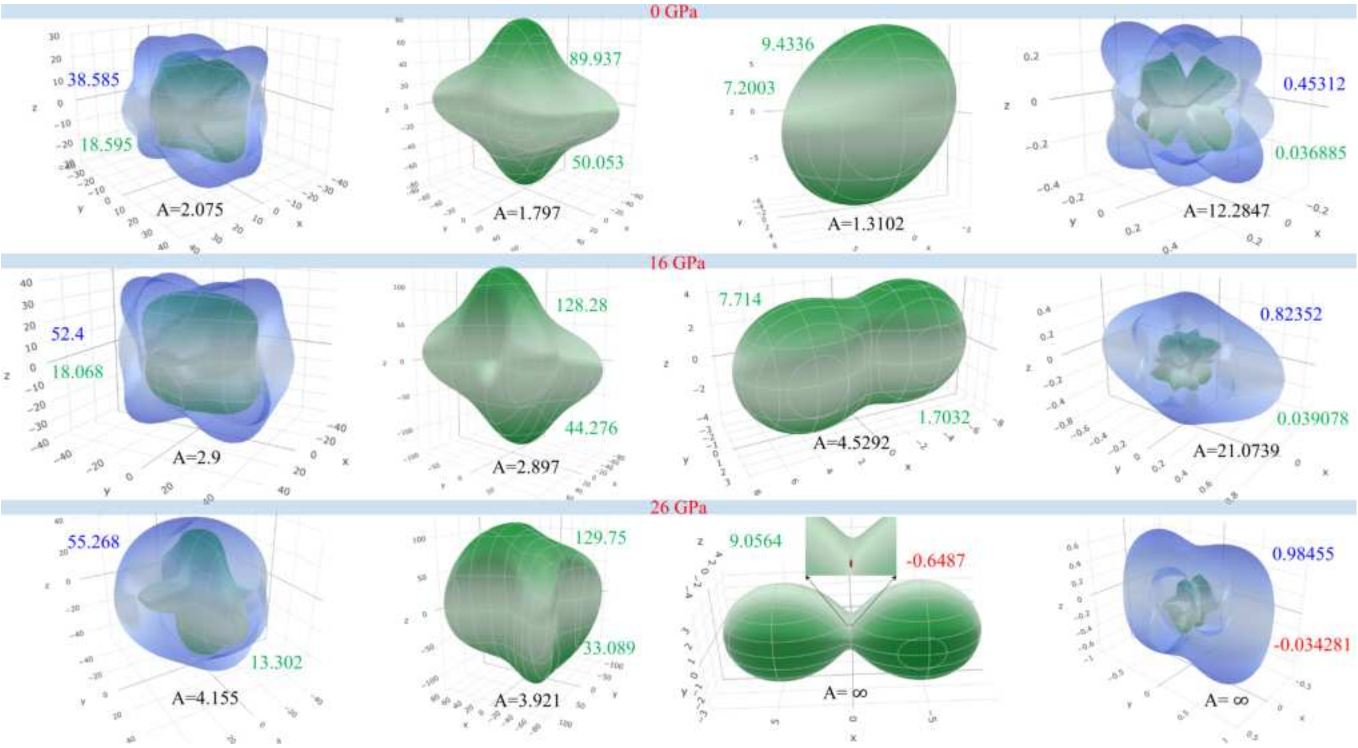


FIG. S4. The 3D form elastic modulus parameters of monoclinic $SrIn_2As_2$ under different pressures include shear modulus $G$, Young's modulus $Y$, linear compression ($LC$), and Poisson's ratio ($v$). The blue and green surfaces indicate the maximum positive and minimum positive values of $G$, and the maximum positive value of $Y$ is indicated by the green surface. The positive values of $LC$ are represented in green surface, and those of negative $LC$ are represented in red surface. For $v$, the maximum (blue), minimum positive (green), and minimum negative (red) values.

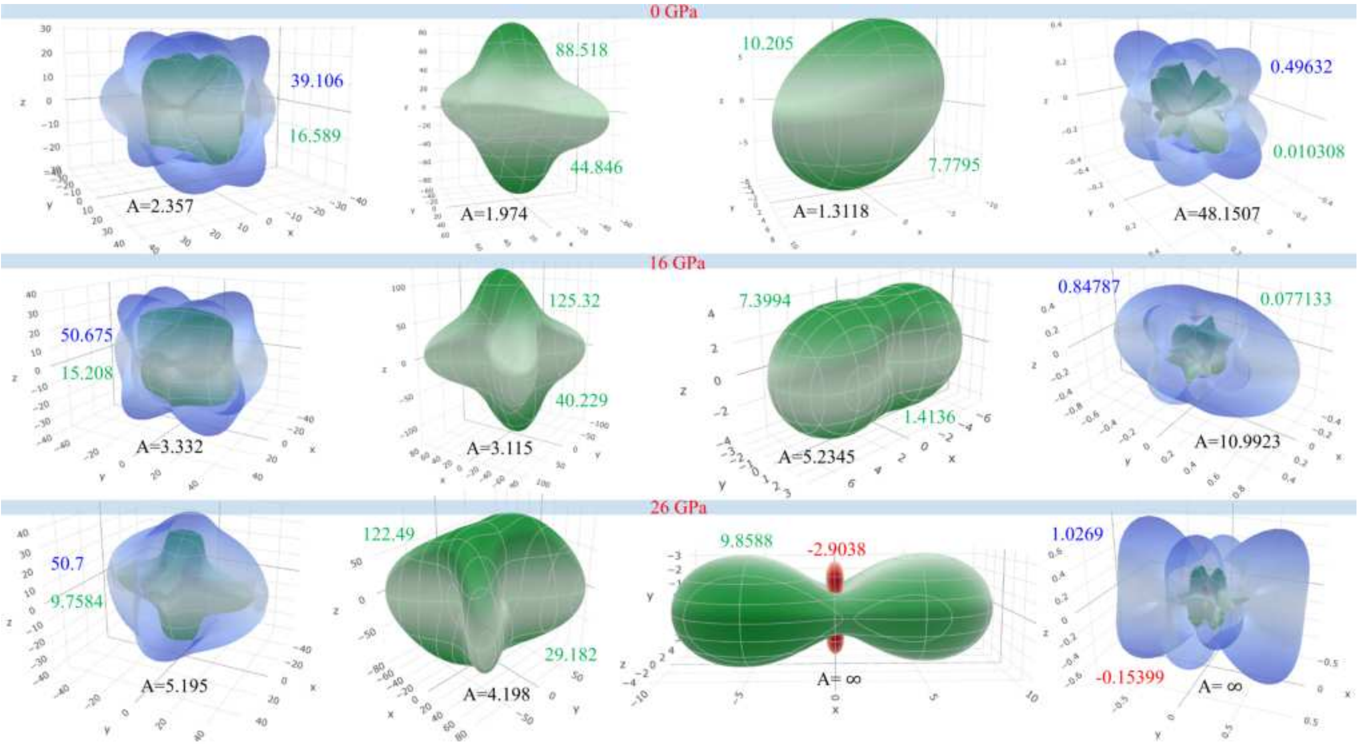


FIG. S5. The 3D form elastic modulus parameters of monoclinic $BaIn_2As_2$ under different pressures include shear modulus $G$, Young's modulus $Y$, linear compression ($LC$), and Poisson's ratio ($v$). The blue and green surfaces indicate the maximum positive and minimum positive values of $G$, and the maximum positive value of $Y$ is indicated by the green surface. The positive values of $LC$ are represented in green surface, and those of negative $LC$ are represented in red surface. For $v$, the maximum (blue), minimum positive (green), and minimum negative (red) values.

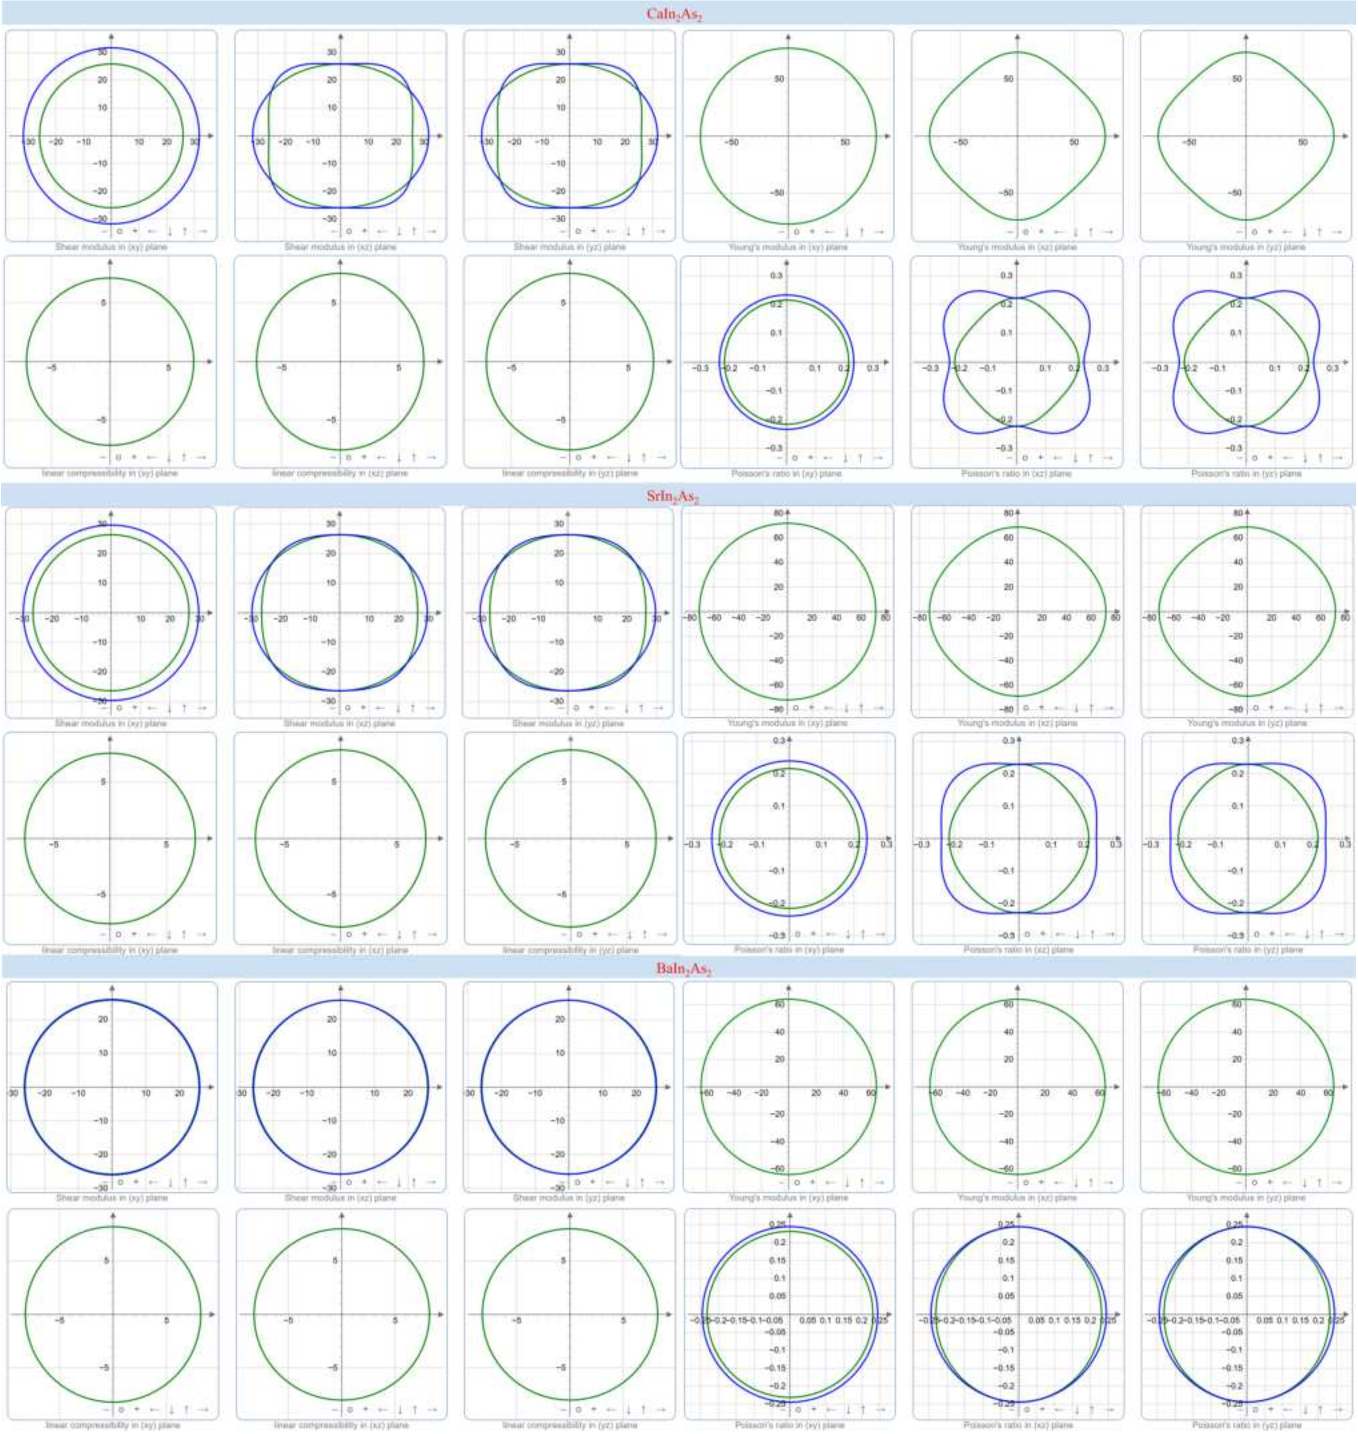


FIG. S6. Elastic modulus parameters of hexagonal ($P6_3/mmc$) AEIn$_2$As$_2$ under 0 GPa in $xy$, $xz$, and $yz$ planes. The shear modulus $G$, Young's modulus $Y$, linear compression ($LC$), and Poisson's ratio ($v$) are given for different pressure cases. The blue and green curves indicate the maximum positive and minimum positive values of $G$, and the maximum positive value of $Y$ is indicated by the green curve. Directions corresponding to positive values of $LC$ are represented in green, and those of negative $LC$ are represented in red. For $v$, the maximum (blue), minimum positive (green), and minimum negative (red) values.

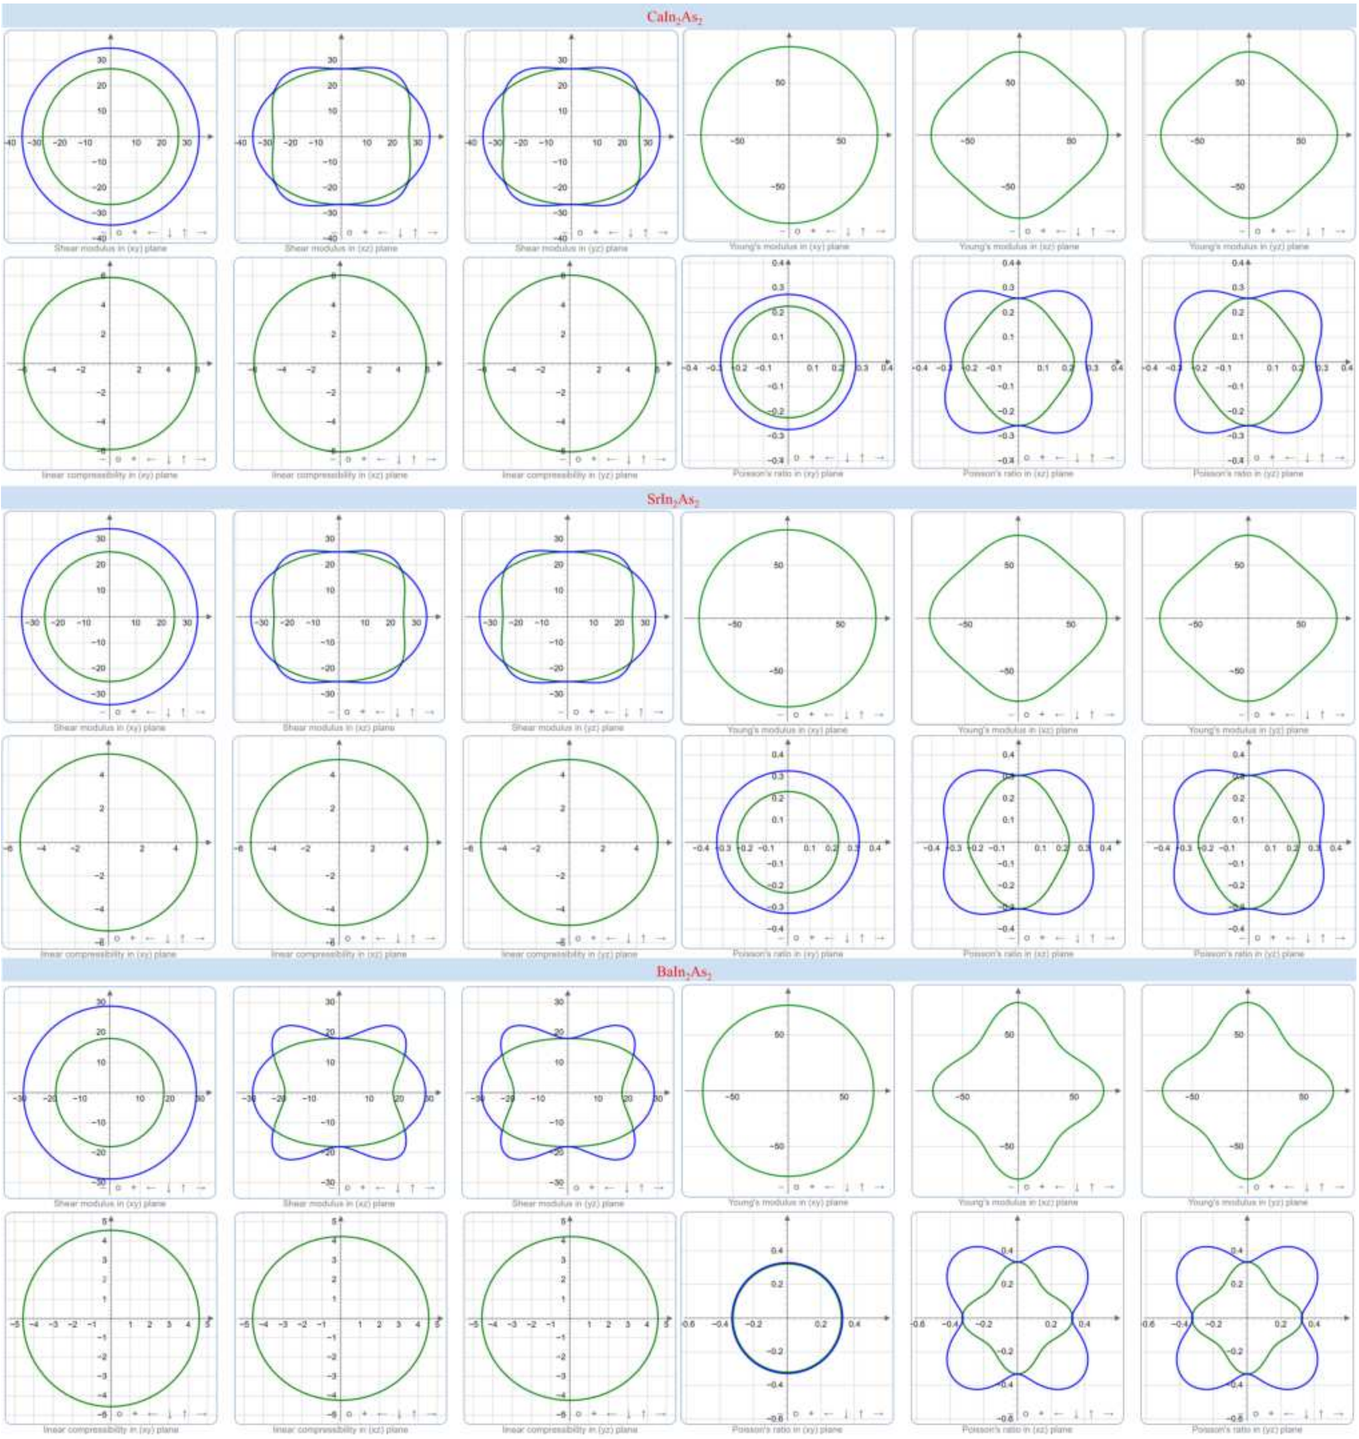


FIG. S7. Elastic modulus parameters of hexagonal ($P6_3/mmc$) $\mathrm{AEIn_2As_2}$ induced zero band gap under pressure in $xy$, $xz$, and $yz$ planes. The shear modulus $G$, Young's modulus $Y$, linear compression ($LC$), and Poisson's ratio ($v$) are given for different pressure cases. The blue and green curves indicate the maximum positive and minimum positive values of $G$, and the maximum positive value of $Y$ is indicated by the green curve. Directions corresponding to positive values of $LC$ are represented in green, and those of negative $LC$ are represented in red. For $v$, the maximum (blue), minimum positive (green), and minimum negative (red) values.

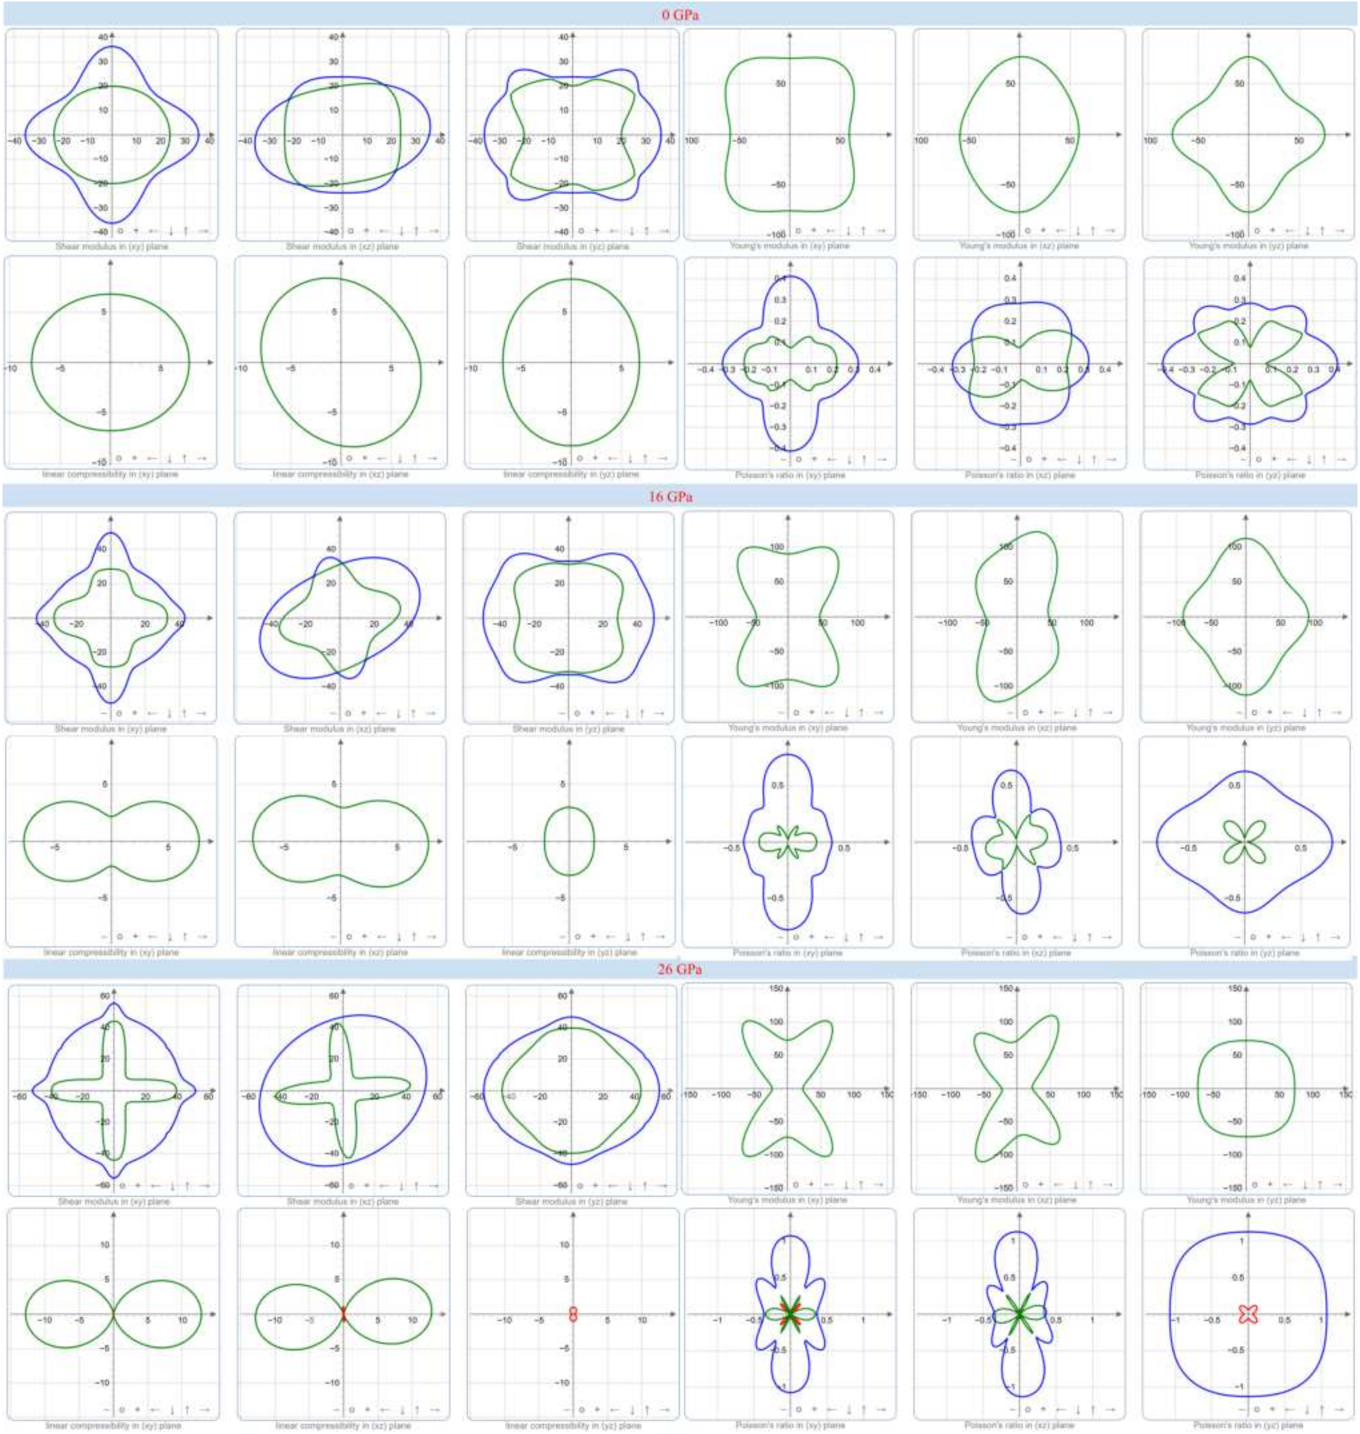


FIG. S8. Elastic modulus parameters of monoclinic $CaIn_2As_2$ at different pressures in $xy$, $xz$, and $yz$ planes. The shear modulus $G$, Young's modulus $Y$, linear compression ($LC$), and Poisson's ratio ($v$) are given for different pressure cases. The blue and green curves indicate the maximum positive and minimum positive values of $G$, and the maximum positive value of $Y$ is indicated by the green curve. Directions corresponding to positive values of $LC$ are represented in green, and those of negative $LC$ are represented in red. For $v$, the maximum (blue), minimum positive (green), and minimum negative (red) values.

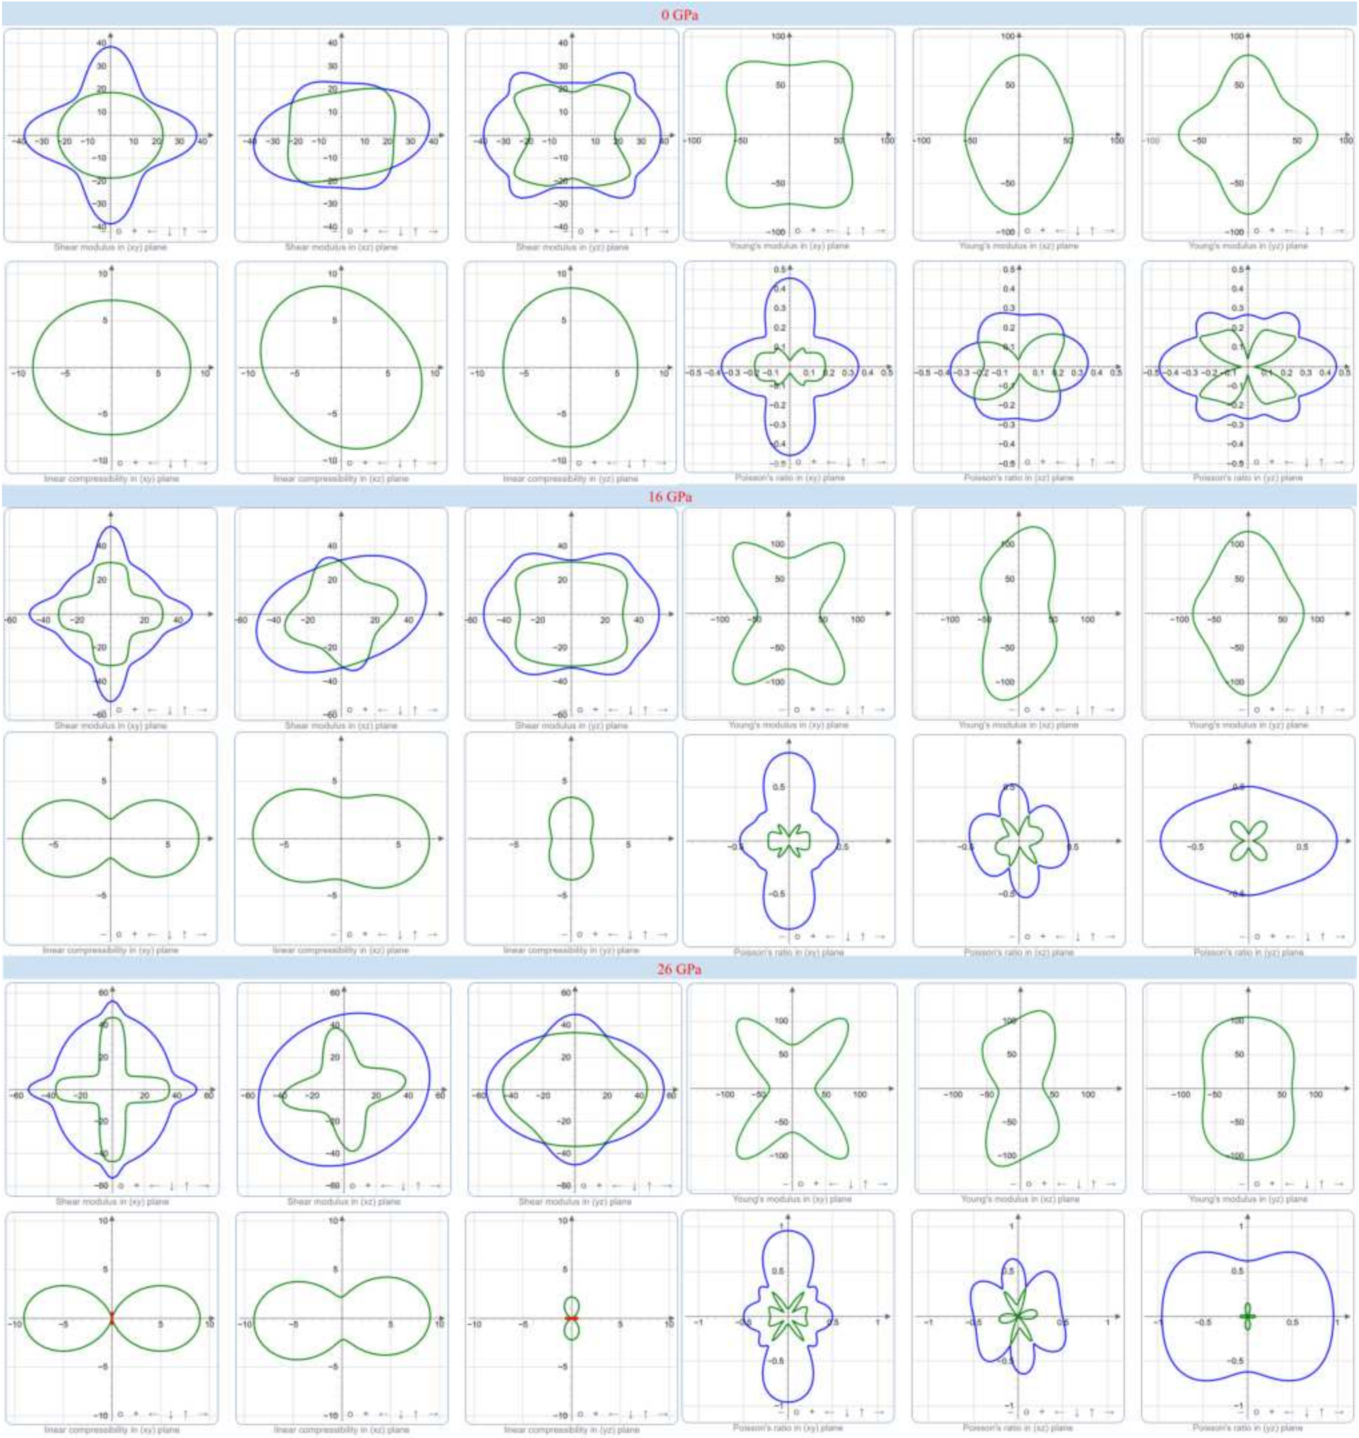


FIG. S9. Elastic modulus parameters of monoclinic $SrIn_2As_2$ at different pressures in $xy$, $xz$, and $yz$ planes. The shear modulus $G$, Young's modulus $Y$, linear compression ($LC$), and Poisson's ratio ($v$) are given for different pressure cases. The blue and green curves indicate the maximum positive and minimum positive values of $G$, and the maximum positive value of $Y$ is indicated by the green curve. Directions corresponding to positive values of $LC$ are represented in green, and those of negative $LC$ are represented in red. For $v$, the maximum (blue), minimum positive (green), and minimum negative (red) values.

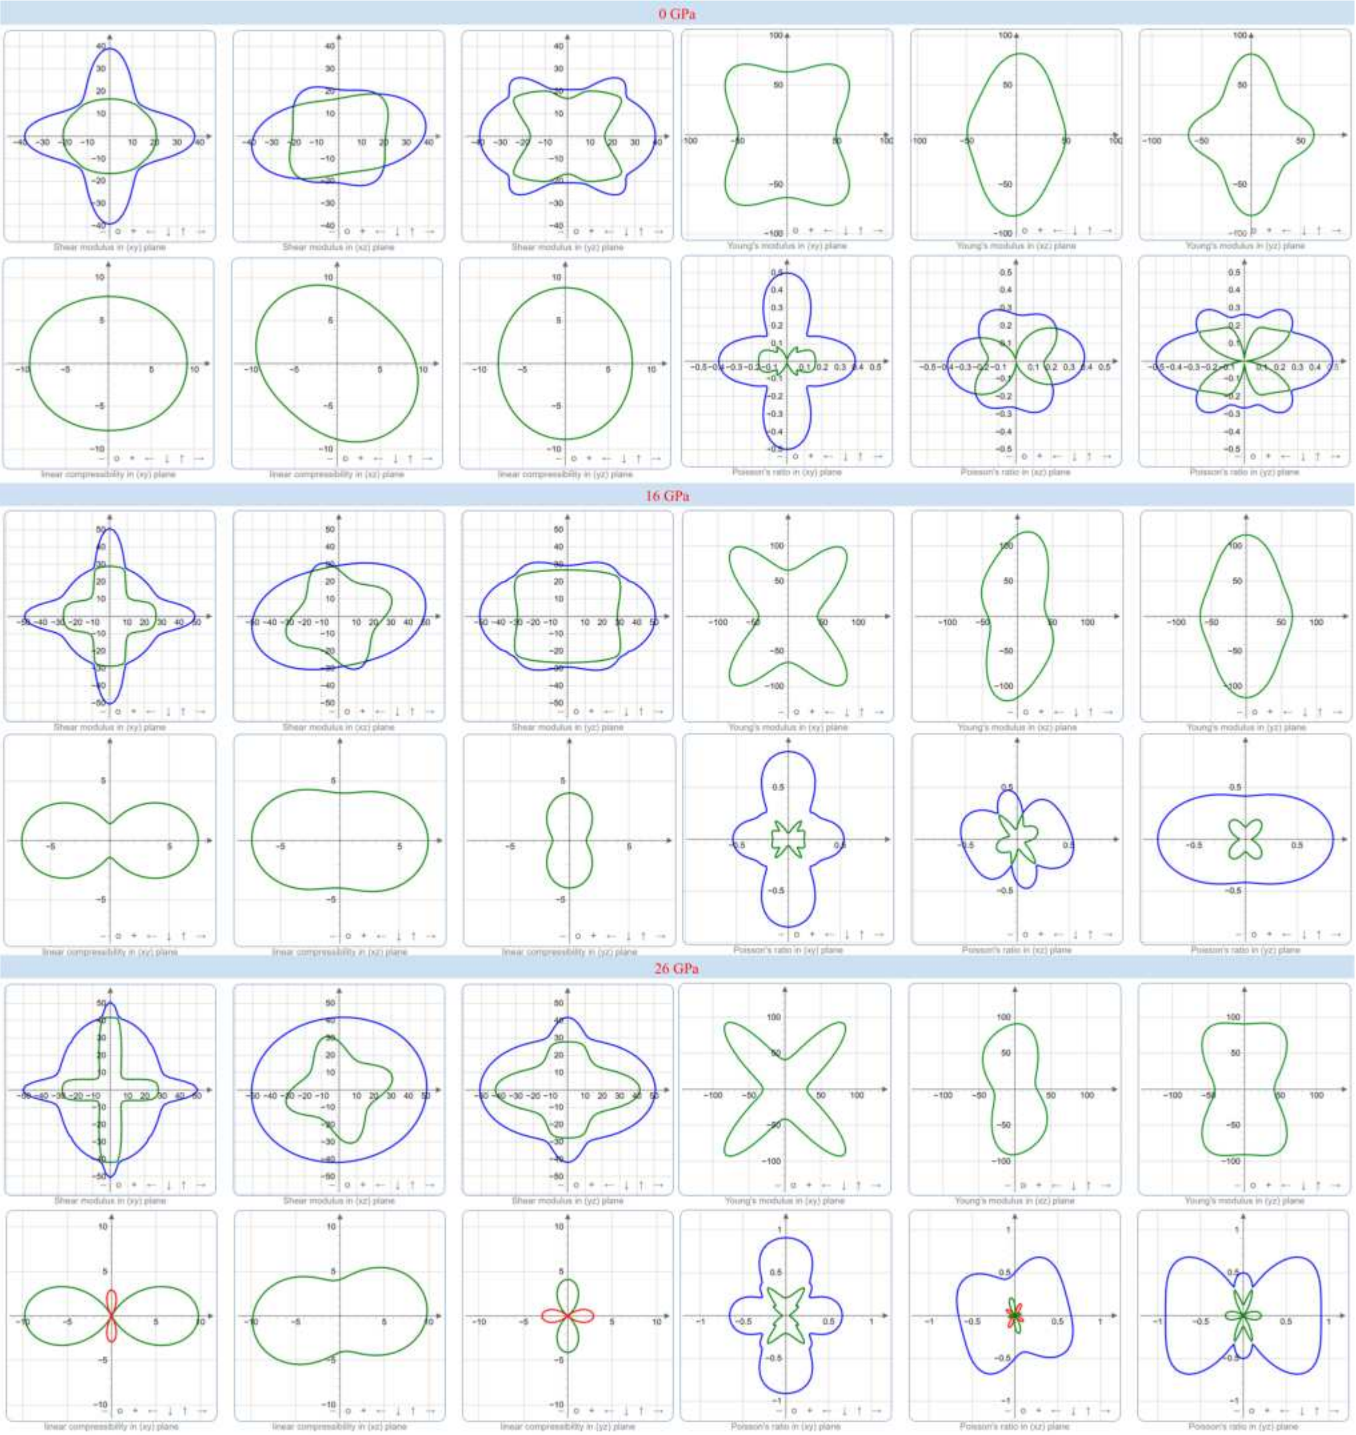


FIG. S10. Elastic modulus parameters of monoclinic $BaIn_2As_2$ at different pressures in $xy$, $xz$, and $yz$ planes. The shear modulus $G$, Young's modulus $Y$, linear compression ($LC$), and Poisson's ratio ($v$) are given for different pressure cases. The blue and green curves indicate the maximum positive and minimum positive values of $G$, and the maximum positive value of $Y$ is indicated by the green curve. Directions corresponding to positive values of $LC$ are represented in green, and those of negative $LC$ are represented in red. For $v$, the maximum (blue), minimum positive (green), and minimum negative (red) values.

## B. Thermal Properties

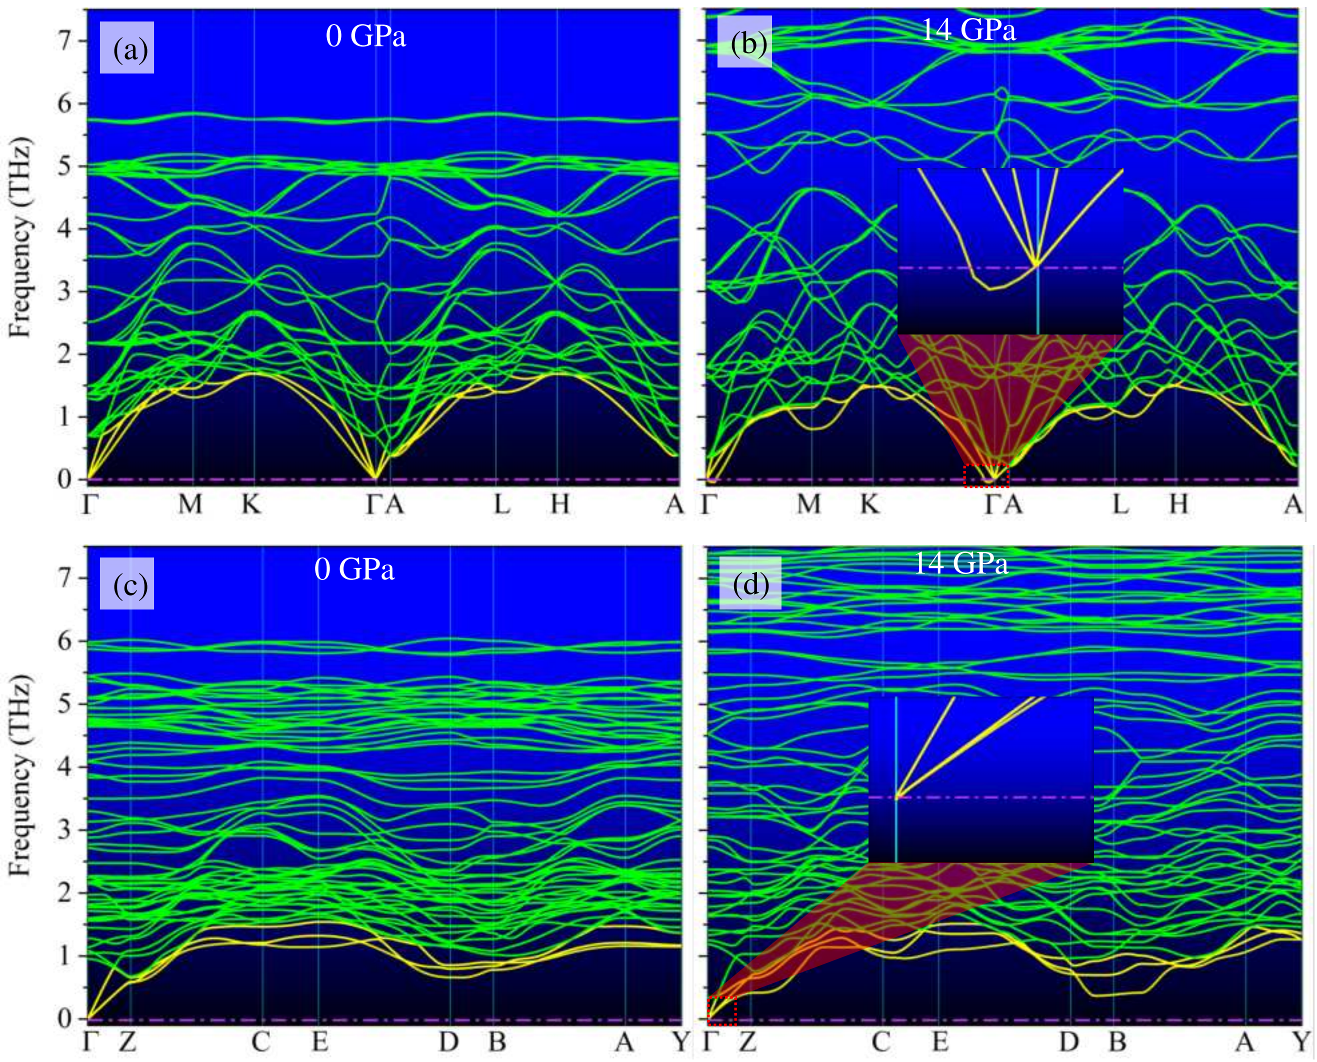


FIG. S11. Phonon dispersion curves with $R\bar{3}m$ space group at (a) atmospheric pressure and (b) 14 GPa. Phonon dispersion curves for the $P2/m$ space group at (c) atmospheric pressure and (d) 14 GPa.

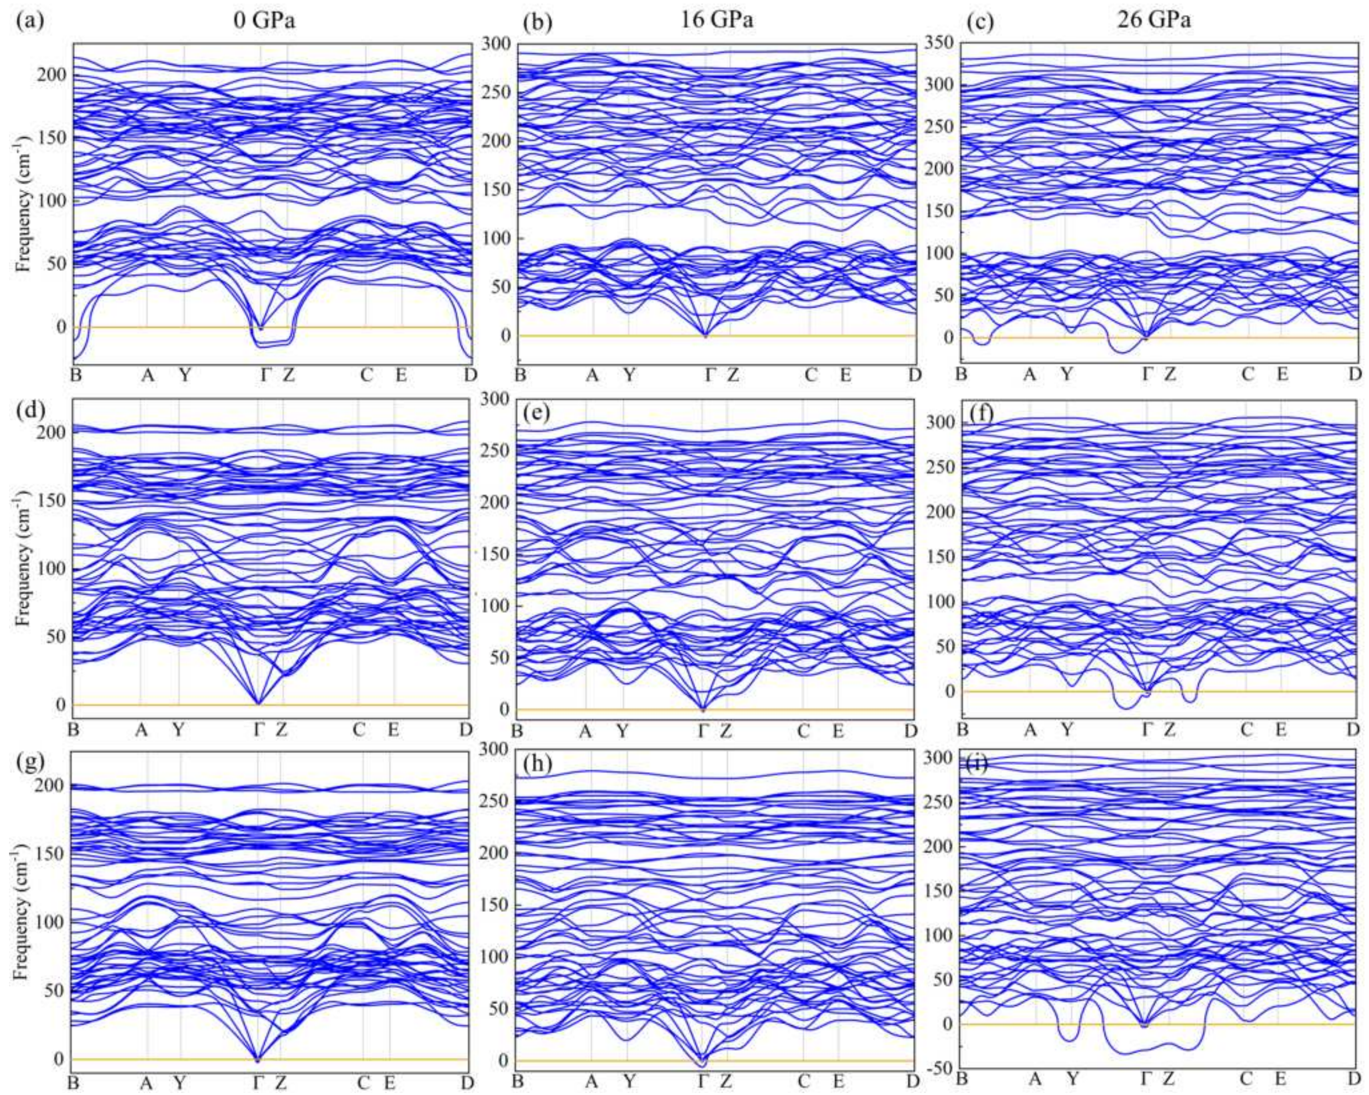


FIG. S12. Phonon dispersion spectra of the monoclinic phase $AEIn_2As_2$ at different pressures. Each row represents the calculated results for $CaIn_2As_2$, $SrIn_2As_2$, and $BaIn_2As_2$. The different pressure values are marked at the top.

TABLE S1. Frequency values of the phonon spectrum of $AEIn_2As_2$ with $P2/m$ phase under different pressures. Frequencies, activities and symmetries are labelled F., A. and S., respectively. Bolded text is relevant at larger imaginary frequencies (frequencies below -3 $cm^{-1}$ (-0.09 THz)).

| $CaIn_2As_2$ | | | | | | | | | $SrIn_2As_2$ | | | | | | | | | $BaIn_2As_2$ | | | | | | | | |
|---|---|---|---|---|---|---|---|---|---|---|---|---|---|---|---|---|---|---|---|---|---|---|---|---|---|---|
| 0GPa | | | 16GPa | | | 26GPa | | | 0GPa | | | 16GPa | | | 26GPa | | | 0GPa | | | 16GPa | | | 26GPa | | |
| F. | A. | S. | F. | A. | S. | F. | A. | S. | F. | A. | S. | F. | A. | S. | F. | A. | S. | F. | A. | S. | F. | A. | S. | F. | A. | S. |
| **-16.00** | **IR** | **Au** | -1.67 | IR | Au | -2.67 | IR | Bu | 0 | IR | Bu | -2.00 | IR | Au | **-6.00** | **IR** | **Bu** | -2.20 | IR | Bu | **-5.67** | **IR** | **Bu** | **-29.00** | **IR** | **Bu** |
| **-12.33** | **R** | **Bg** | -1.33 | IR | Bu | -0.33 | IR | Au | 0 | IR | Au | -1.33 | IR | Bu | -1.67 | IR | Au | -1.54 | IR | Au | -1.00 | IR | Bu | **-3.00** | **IR** | **Bu** |
| -2.33 | IR | Bu | -0.67 | IR | Bu | -0.33 | IR | Bu | 0 | IR | Bu | 0 | IR | Bu | -1.00 | IR | Bu | -0.86 | IR | Bu | -1.00 | IR | Au | -1.00 | IR | Au |
| -0.95 | IR | Bu | 21.40 | IR | Bu | 6.93 | IR | Bu | 36.87 | IR | Bu | 17.26 | IR | Bu | 10.32 | IR | Bu | 31.96 | R | Ag | 6.56 | IR | Bu | 0.23 | IR | Bu |
| 34.41 | IR | Au | 42.16 | IR | Au | 29.20 | IR | Bu | 36.93 | R | Ag | 39.59 | IR | Au | 33.20 | IR | Bu | 33.98 | R | Bg | 36.76 | IR | Au | 30.95 | IR | Bu |
| 35.24 | R | Ag | 42.51 | IR | Bu | 45.06 | IR | Au | 39.77 | R | Bg | 43.38 | R | Ag | 43.63 | IR | Au | 34.60 | IR | Bu | 43.21 | R | Ag | 40.92 | IR | Au |
| 37.40 | IR | Bu | 43.91 | R | Ag | 47.50 | R | Ag | 40.59 | IR | Au | 43.42 | R | Bg | 45.13 | R | Ag | 35.75 | IR | Au | 43.31 | R | Bg | 43.06 | R | Ag |
| 41.99 | IR | Au | 46.35 | R | Bg | 54.29 | R | Bg | 45.69 | IR | Bu | 45.92 | IR | Bu | 53.19 | R | Bg | 42.65 | IR | Bu | 46.83 | IR | Bu | 50.96 | R | Bg |
| 43.72 | IR | Bu | 46.95 | IR | Au | 57.35 | IR | Au | 50.43 | IR | Au | 52.39 | IR | Au | 61.45 | R | Bg | 47.81 | IR | Au | 54.90 | IR | Au | 55.85 | IR | Bu |
| 51.04 | R | Bg | 52.57 | IR | Bu | 62.87 | R | Bg | 55.35 | R | Ag | 57.60 | IR | Bu | 62.28 | IR | Au | 51.30 | R | Bg | 55.09 | IR | Bu | 59.21 | R | Bg |
| 56.65 | R | Ag | 60.24 | R | Ag | 63.01 | IR | Bu | 55.42 | R | Bg | 58.02 | R | Ag | 63.06 | IR | Bu | 51.95 | R | Ag | 56.78 | R | Ag | 63.60 | IR | Au |
| 57.05 | IR | Au | 62.84 | R | Bg | 67.57 | R | Ag | 58.06 | IR | Bu | 60.44 | R | Bg | 69.86 | R | Ag | 54.00 | IR | Bu | 58.64 | R | Bg | 63.99 | R | Ag |
| 58.58 | R | Bg | 64.57 | IR | Bu | 71.04 | R | Bg | 59.67 | R | Ag | 64.56 | IR | Bu | 70.92 | R | Bg | 56.53 | R | Ag | 65.15 | R | Bg | 70.08 | R | Bg |
| 58.81 | IR | Bu | 66.91 | R | Bg | 72.18 | IR | Bu | 60.01 | R | Bg | 66.49 | R | Bg | 78.47 | IR | Bu | 58.31 | IR | Au | 67.96 | IR | Bu | 72.28 | IR | Bu |
| 61.28 | R | Ag | 70.20 | IR | Au | 77.55 | IR | Au | 61.43 | IR | Au | 69.77 | IR | Au | 79.13 | IR | Au | 58.90 | R | Bg | 68.04 | IR | Au | 77.97 | IR | Au |
| 63.00 | R | Bg | 73.26 | R | Bg | 81.21 | IR | Bu | 64.37 | IR | Bu | 77.38 | R | Ag | 79.86 | IR | Bu | 61.07 | IR | Bu | 74.16 | R | Ag | 79.18 | IR | Bu |
| 64.21 | IR | Bu | 78.75 | R | Ag | 83.08 | R | Ag | 64.87 | R | Bg | 79.56 | IR | Bu | 84.37 | R | Ag | 62.80 | R | Bg | 77.08 | IR | Bu | 81.59 | R | Ag |
| 68.48 | R | Ag | 82.11 | IR | Bu | 87.02 | R | Bg | 71.51 | R | Ag | 79.70 | R | Bg | 91.94 | R | Ag | 66.07 | IR | Bu | 81.00 | R | Bg | 90.67 | R | Ag |
| 77.23 | IR | Bu | 90.53 | R | Ag | 91.35 | R | Ag | 72.90 | IR | Bu | 91.81 | R | Ag | 93.48 | R | Bg | 71.18 | R | Bg | 92.34 | R | Ag | 95.71 | R | Bg |
| 92.06 | R | Ag | 91.48 | R | Ag | 102.02 | R | Ag | 81.10 | IR | Bu | 96.06 | R | Ag | 105.62 | R | Ag | 71.36 | IR | Au | 97.91 | IR | Bu | 104.82 | R | Ag |
| 105.02 | IR | Bu | 128.96 | IR | Bu | 142.83 | IR | Bu | 85.35 | R | Ag | 108.66 | IR | Bu | 149.08 | IR | Bu | 72.23 | IR | Bu | 98.03 | R | Ag | 114.23 | IR | Bu |
| 106.00 | R | Ag | 141.39 | R | Ag | 147.06 | R | Ag | 85.54 | R | Bg | 122.13 | R | Ag | 150.81 | R | Ag | 72.75 | R | Ag | 111.12 | IR | Au | 122.15 | R | Ag |
| 108.91 | IR | Bu | 149.96 | IR | Bu | 153.53 | IR | Bu | 86.04 | IR | Bu | 129.54 | R | Bg | 159.34 | IR | Bu | 73.09 | IR | Bu | 111.44 | R | Bg | 128.95 | IR | Bu |
| 117.25 | R | Bg | 154.80 | R | Ag | 162.63 | R | Ag | 86.68 | IR | Au | 129.89 | IR | Au | 168.81 | R | Ag | 75.44 | IR | Au | 111.44 | R | Ag | 129.54 | IR | Au |
| 118.34 | IR | Au | 159.90 | R | Bg | 170.38 | R | Ag | 90.39 | IR | Au | 132.16 | IR | Bu | 172.28 | R | Ag | 75.73 | R | Ag | 115.70 | IR | Bu | 133.07 | R | Bg |
| 119.85 | R | Ag | 160.93 | IR | Au | 176.96 | IR | Au | 95.41 | R | Ag | 143.10 | IR | Au | 177.81 | IR | Bu | 81.99 | IR | Au | 123.18 | IR | Au | 135.39 | IR | Au |
| 124.23 | IR | Au | 166.03 | R | Ag | 179.19 | IR | Bu | 99.19 | IR | Au | 144.48 | R | Ag | 179.82 | R | Ag | 90.68 | R | Ag | 128.62 | R | Ag | 141.35 | R | Ag |
| 124.95 | IR | Bu | 167.69 | IR | Bu | 179.44 | R | Bg | 103.92 | IR | Bu | 151.30 | IR | Au | 184.18 | IR | Au | 92.55 | IR | Bu | 129.86 | IR | Au | 147.25 | IR | Bu |
| 127.32 | IR | Bu | 171.96 | R | Ag | 181.71 | R | Ag | 107.03 | R | Ag | 154.25 | IR | Bu | 186.37 | R | Bg | 95.62 | R | Ag | 139.07 | IR | Bu | 153.92 | IR | Bu |
| 130.47 | IR | Au | 174.99 | IR | Au | 181.85 | IR | Au | 112.23 | IR | Bu | 158.25 | R | Ag | 190.28 | IR | Au | 98.69 | IR | Bu | 143.55 | IR | Bu | 158.50 | IR | Au |
| 131.63 | R | Ag | 180.36 | IR | Bu | 182.26 | IR | Bu | 118.36 | R | Ag | 159.52 | IR | Bu | 191.35 | IR | Bu | 104.40 | IR | Bu | 145.28 | IR | Bu | 160.17 | IR | Bu |
| 134.90 | R | Ag | 185.87 | IR | Au | 197.89 | IR | Bu | 123.88 | IR | Bu | 162.40 | R | Ag | 199.51 | IR | Bu | 109.91 | IR | Bu | 153.91 | R | Ag | 164.36 | R | Ag |
| 136.31 | IR | Bu | 185.89 | IR | Bu | 199.39 | IR | Bu | 125.83 | IR | Bu | 163.24 | IR | Bu | 203.05 | IR | Bu | 116.51 | R | Ag | 155.85 | IR | Bu | 174.65 | R | Ag |
| 147.33 | R | Ag | 186.01 | R | Ag | 205.65 | R | Ag | 131.76 | R | Ag | 174.43 | R | Ag | 206.38 | R | Ag | 127.91 | R | Ag | 161.42 | R | Ag | 175.13 | IR | Bu |
| 149.31 | IR | Bu | 195.36 | IR | Bu | 208.74 | R | Ag | 133.20 | IR | Bu | 174.56 | IR | Bu | 211.12 | IR | Bu | 129.24 | IR | Bu | 168.93 | R | Ag | 180.08 | R | Ag |
| 151.90 | R | Ag | 200.08 | IR | Bu | 215.49 | IR | Bu | 139.82 | R | Ag | 180.33 | IR | Bu | 211.67 | R | Ag | 135.80 | R | Ag | 169.37 | IR | Bu | 182.08 | IR | Bu |
| 155.31 | R | Ag | 203.78 | R | Ag | 217.09 | IR | Au | 140.95 | IR | Bu | 185.42 | IR | Bu | 219.74 | R | Ag | 136.73 | IR | Bu | 177.28 | IR | Bu | 185.25 | IR | Bu |
| 155.85 | R | Bg | 211.26 | R | Ag | 218.34 | R | Ag | 144.63 | IR | Bu | 198.58 | R | Ag | 224.05 | IR | Au | 141.37 | R | Ag | 185.27 | R | Ag | 188.88 | R | Ag |
| 157.13 | IR | Bu | 213.21 | R | Bg | 227.17 | R | Bg | 146.61 | R | Ag | 206.68 | IR | Bu | 231.63 | R | Bg | 144.13 | IR | Bu | 196.73 | IR | Bu | 200.74 | IR | Bu |
| 158.60 | IR | Bu | 214.73 | IR | Au | 232.10 | IR | Au | 155.45 | R | Ag | 206.76 | R | Ag | 236.80 | IR | Au | 153.65 | R | Bg | 199.51 | R | Ag | 209.57 | R | Ag |
| 159.07 | R | Bg | 217.95 | R | Ag | 232.99 | R | Bg | 157.07 | R | Bg | 207.80 | R | Ag | 238.10 | R | Ag | 154.10 | IR | Au | 207.19 | R | Ag | 212.10 | R | Ag |
| 159.45 | IR | Au | 218.17 | IR | Bu | 237.02 | IR | Bu | 158.73 | IR | Au | 210.73 | R | Bg | 241.15 | R | Bg | 154.92 | IR | Bu | 209.39 | IR | Bu | 216.28 | IR | Bu |
| 162.18 | IR | Bu | 221.79 | R | Bg | 237.29 | R | Ag | 159.58 | R | Bg | 211.11 | IR | Au | 242.56 | IR | Bu | 155.83 | R | Bg | 212.27 | R | Ag | 218.34 | R | Ag |
| 165.62 | R | Bg | 228.24 | IR | Bu | 243.78 | IR | Bu | 160.45 | IR | Bu | 216.08 | R | Ag | 243.52 | R | Ag | 156.34 | IR | Au | 213.15 | IR | Au | 229.95 | R | Bg |
| 165.86 | IR | Au | 228.63 | R | Ag | 244.67 | R | Ag | 161.13 | IR | Au | 218.10 | IR | Bu | 251.07 | IR | Bu | 157.27 | R | Ag | 213.21 | R | Bg | 230.08 | IR | Au |
| 165.93 | R | Ag | 232.72 | R | Bg | 254.96 | R | Ag | 163.59 | R | Ag | 225.32 | R | Bg | 262.24 | IR | Bu | 158.94 | R | Ag | 220.49 | IR | Bu | 232.44 | IR | Bu |
| 166.85 | IR | Bu | 237.96 | R | Ag | 254.99 | IR | Bu | 165.43 | IR | Bu | 227.59 | IR | Au | 262.92 | R | Ag | 161.28 | IR | Bu | 225.09 | IR | Au | 242.77 | R | Bg |
| 172.46 | IR | Au | 240.82 | IR | Bu | 270.74 | R | Bg | 168.24 | IR | Au | 227.74 | IR | Bu | 276.06 | R | Ag | 162.64 | IR | Au | 225.51 | R | Bg | 243.38 | IR | Au |
| 172.69 | R | Bg | 245.08 | IR | Au | 274.38 | R | Ag | 168.26 | IR | Bu | 230.62 | R | Bg | 278.56 | R | Bg | 162.65 | R | Bg | 227.25 | IR | Bu | 249.93 | IR | Bu |
| 174.18 | IR | Bu | 247.03 | R | Bg | 275.47 | R | Ag | 168.33 | R | Bg | 233.06 | IR | Bu | 282.04 | IR | Au | 164.60 | IR | Bu | 235.00 | R | Bg | 251.67 | R | Bg |
| 174.25 | R | Ag | 251.93 | IR | Bu | 278.21 | IR | Bu | 169.19 | R | Bg | 238.67 | R | Ag | 287.07 | R | Bg | 166.55 | R | Ag | 236.27 | R | Ag | 253.91 | R | Ag |

| | | | | | | | | | | | | | | | | | | | | | | | | | | |
|---|---|---|---|---|---|---|---|---|---|---|---|---|---|---|---|---|---|---|---|---|---|---|---|---|---|---|
| 175.75 | IR | Bu | 256.22 | IR | Bu | 278.22 | IR | Au | 171.16 | R | Ag | 241.31 | IR | Au | 287.85 | IR | Bu | 167.87 | R | Bg | 239.48 | IR | Bu | 258.97 | IR | Au |
| 180.28 | IR | Bu | 258.48 | R | Ag | 280.92 | R | Bg | 173.49 | IR | Au | 243.37 | R | Bg | 288.92 | R | Ag | 168.93 | IR | Au | 240.80 | IR | Au | 260.40 | IR | Bu |
| 180.82 | IR | Au | 263.25 | R | Ag | 289.21 | IR | Bu | 173.51 | IR | Bu | 248.58 | IR | Bu | 298.98 | IR | Bu | 170.19 | IR | Bu | 245.26 | R | Bg | 262.82 | IR | Bu |
| 182.50 | R | Ag | 266.05 | IR | Bu | 289.47 | IR | Bu | 182.23 | R | Ag | 250.50 | IR | Bu | 300.43 | R | Ag | 179.70 | R | Ag | 246.06 | IR | Bu | 266.41 | R | Ag |
| 191.83 | R | Ag | 266.13 | R | Ag | 293.45 | R | Ag | 186.68 | IR | Bu | 251.62 | R | Ag | 302.13 | IR | Au | 180.70 | IR | Bu | 250.59 | IR | Au | 272.18 | R | Ag |
| 197.86 | IR | Bu | 266.95 | IR | Au | 294.03 | IR | Au | 186.71 | R | Ag | 255.08 | IR | Au | 310.63 | IR | Bu | 182.42 | R | Ag | 250.68 | R | Ag | 276.40 | IR | Bu |
| 203.40 | IR | Bu | 271.43 | IR | Au | 313.59 | IR | Bu | 200.06 | IR | Bu | 255.95 | R | Ag | 326.71 | IR | Bu | 196.35 | IR | Bu | 251.11 | R | Ag | 285.87 | R | Bg |
| 204.95 | R | Ag | 275.29 | IR | Bu | 322.64 | IR | Au | 203.16 | R | Ag | 258.25 | IR | Bu | 337.05 | IR | Au | 198.46 | R | Ag | 253.02 | IR | Bu | 294.46 | IR | Au |
| 205.51 | R | Ag | 289.33 | IR | Bu | 329.10 | IR | Bu | 203.57 | R | Ag | 268.76 | R | Ag | 341.52 | IR | Bu | 199.96 | R | Ag | 272.00 | R | Ag | 296.74 | R | Ag |

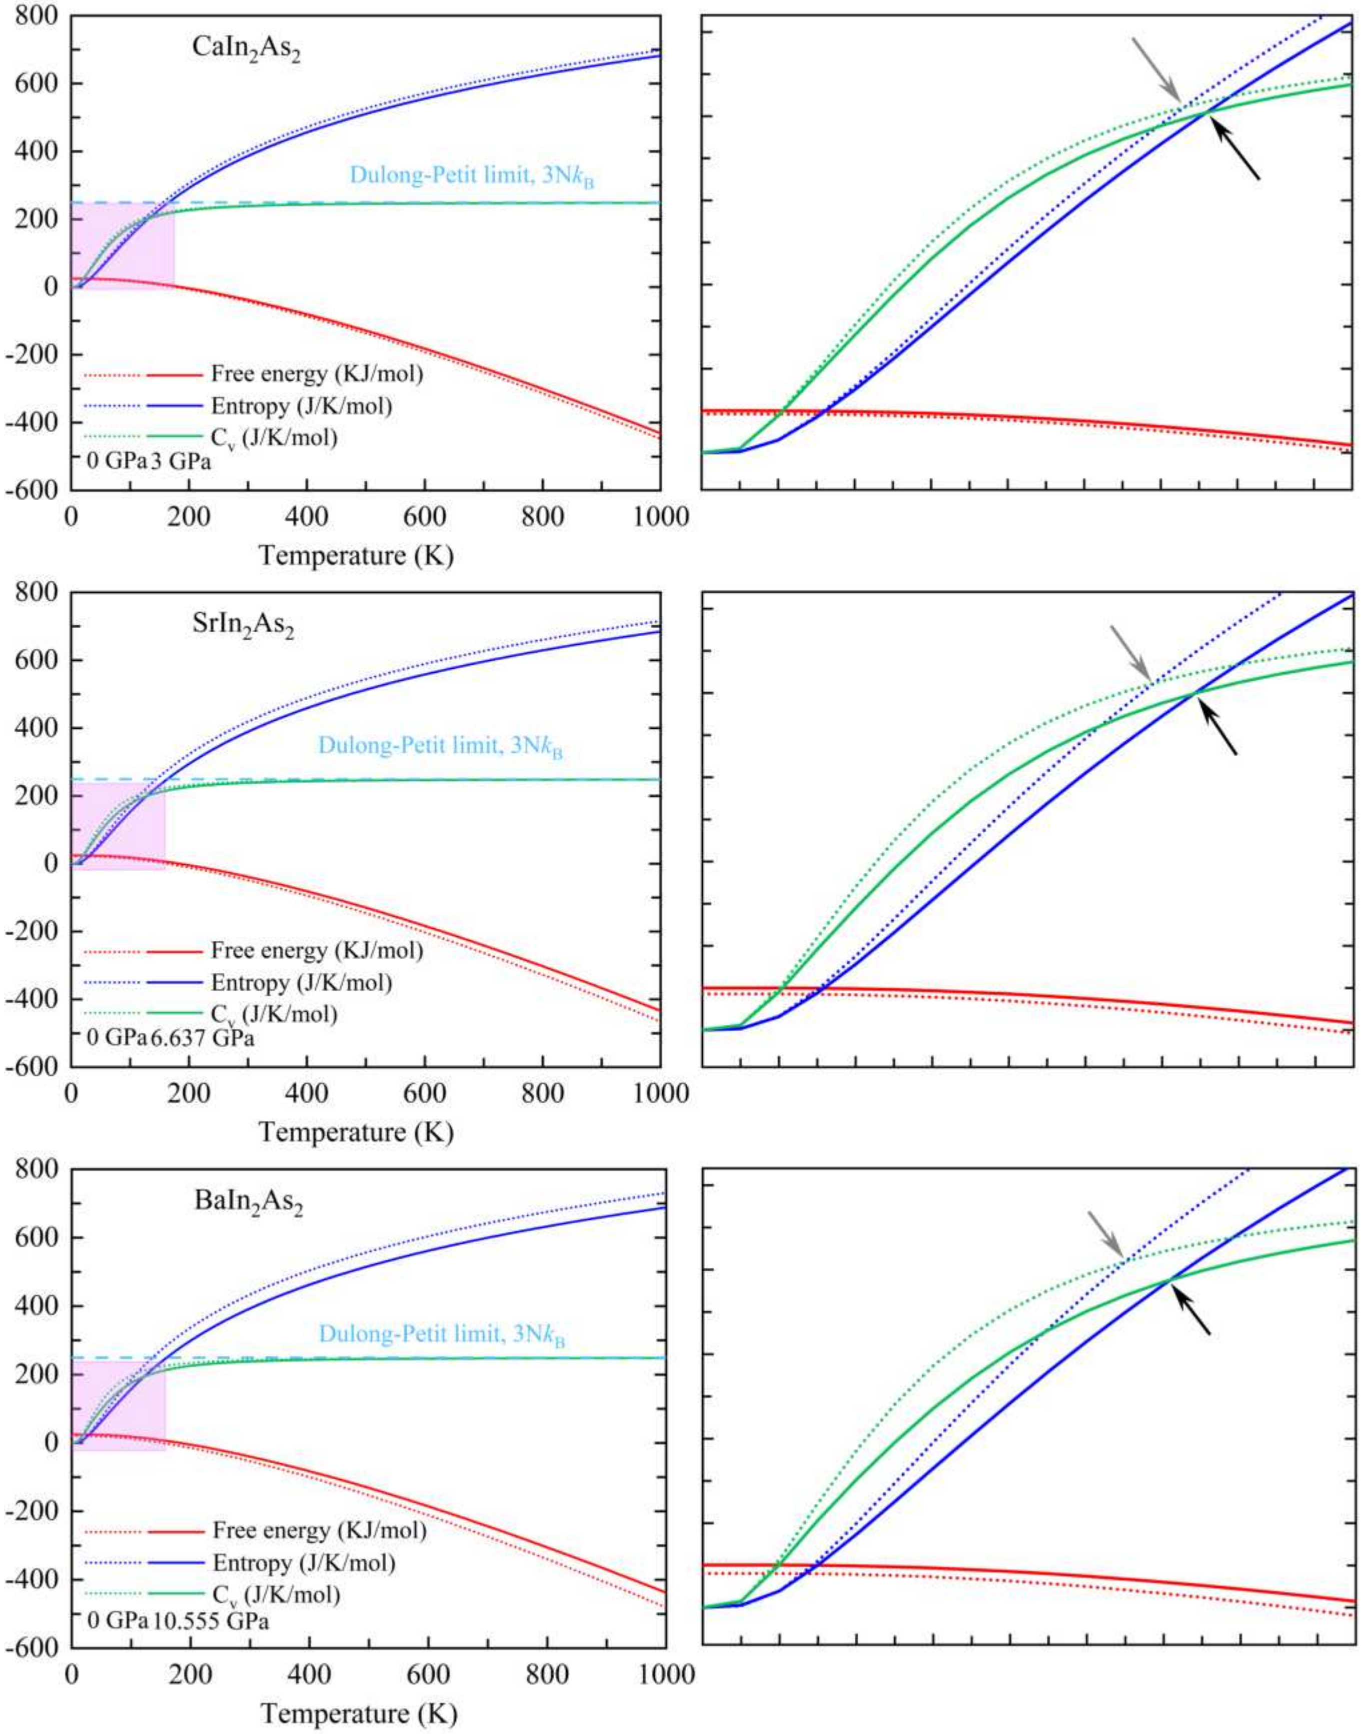


FIG. S13. Temperature-dependent thermodynamic curves of $AEIn_2As_2$ for the $P6_3/mmc$ space group under zero pressure and induced zero bandgap pressure. Each row represents the calculated results for $CaIn_2As_2$, $SrIn_2As_2$, and $BaIn_2As_2$. The heat capacity $C_V$, entropy $S$, and free energy $F$ are included. The second column corresponds to the shaded enlargement of the first column.

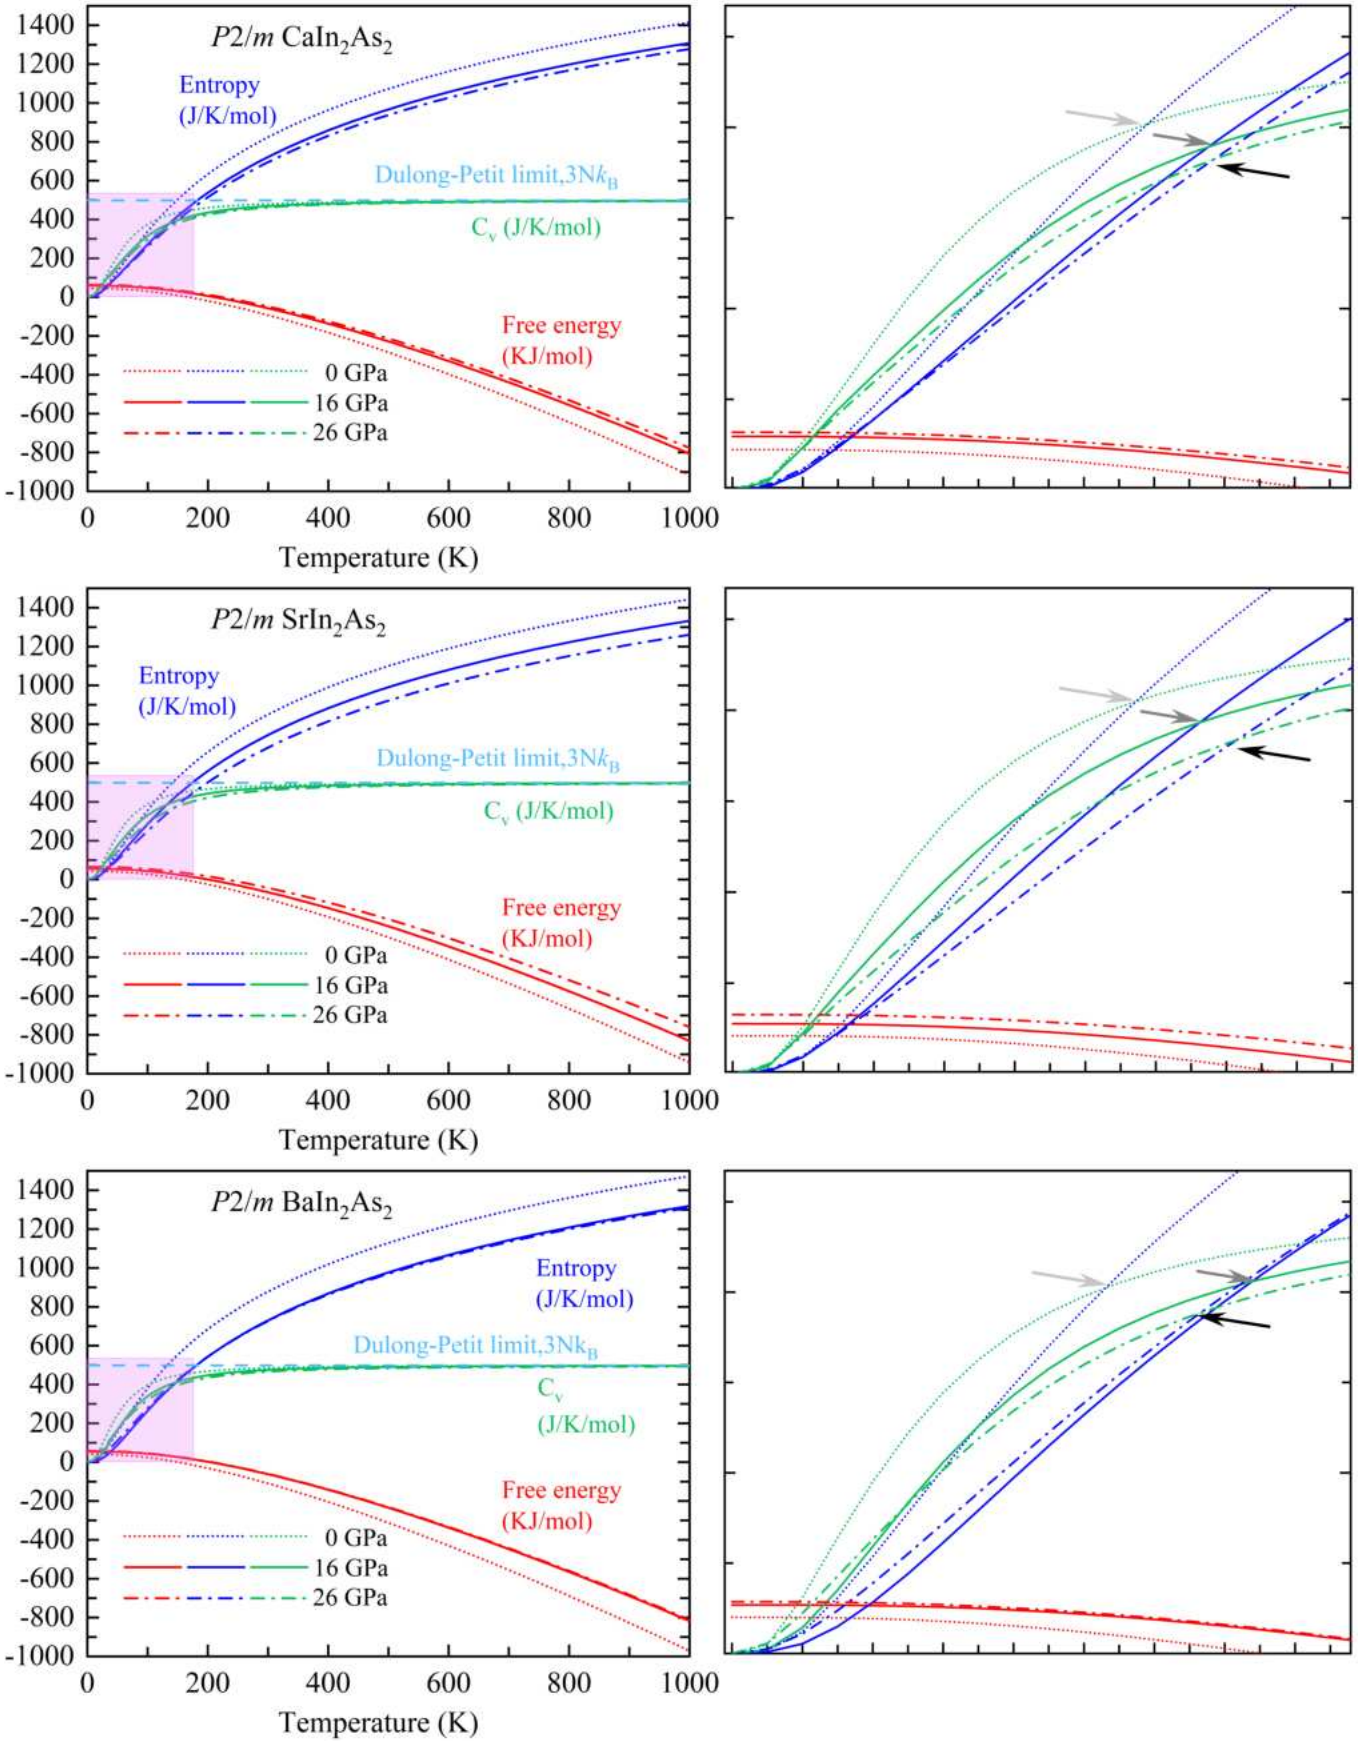


FIG. S14. Temperature-dependent thermodynamic curves of $AEIn_2As_2$ for the $P2/m$ space group under different pressures. Each row represents the calculated results for $CaIn_2As_2$, $SrIn_2As_2$, and $BaIn_2As_2$. The heat capacity $C_V$, entropy $S$, and free energy $F$ are included. The second column corresponds to the shaded enlargement of the first column.

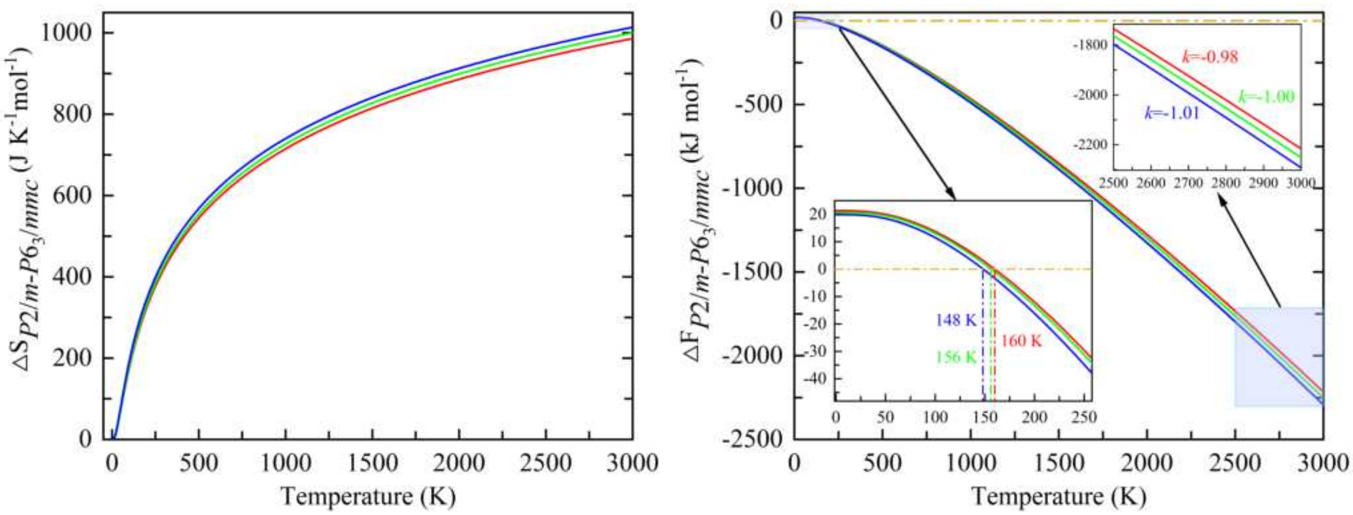


FIG. S15. The monoclinic ($P2/m$) and hexagonal phases ($P6_3/mmc$) depend on the entropy difference $\Delta S$ in temperature and the Helmholtz free energy difference $\Delta F$. Where $\Delta F > 0$ represents a tendency to form a hexagonal phase, while $\Delta F < 0$ tends to present a monoclinic phase.

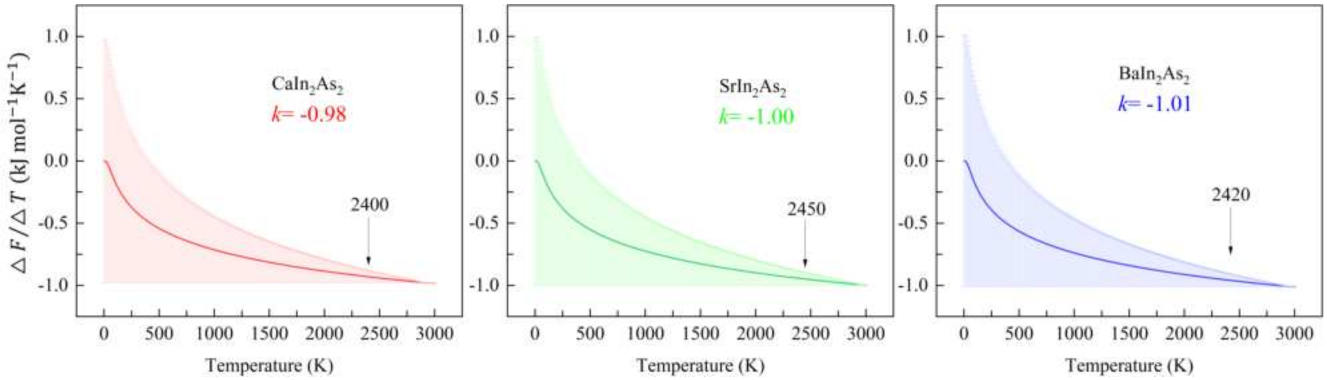


FIG. S16. Rate of change of the free energy of the monoclinic phase $AEIn_2As_2$ with temperature in the absence of pressure. The solid line indicates the actual slope of the curve in Fig. S15(b), and the filled part indicates the deviation from the labeled linear slope at high temperatures. The post-temperature error indicated by the arrows is less than 5%, essentially linear.

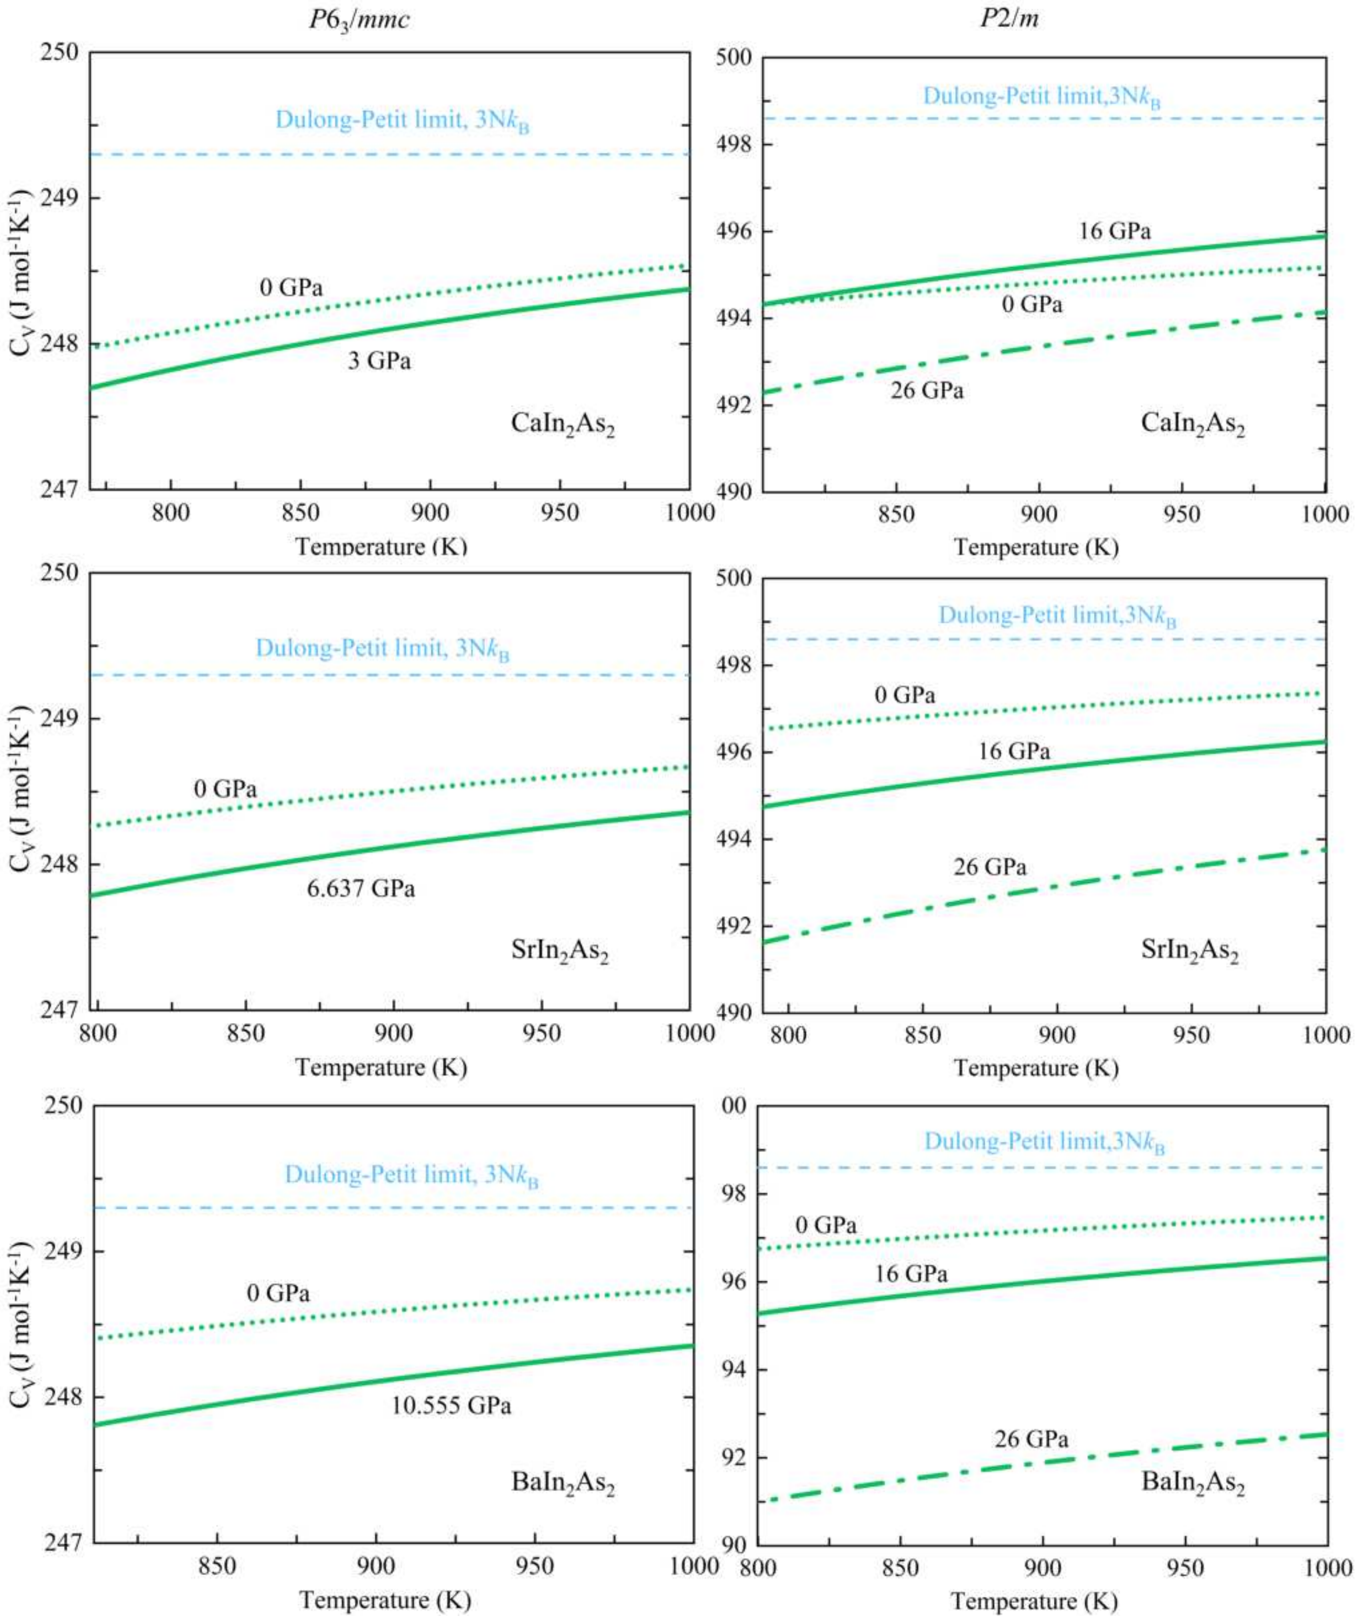


FIG. S17. Heat capacity curves of AEIn for two space groups at different pressures near 1000 K, approximating the Dulong-Petit limit.

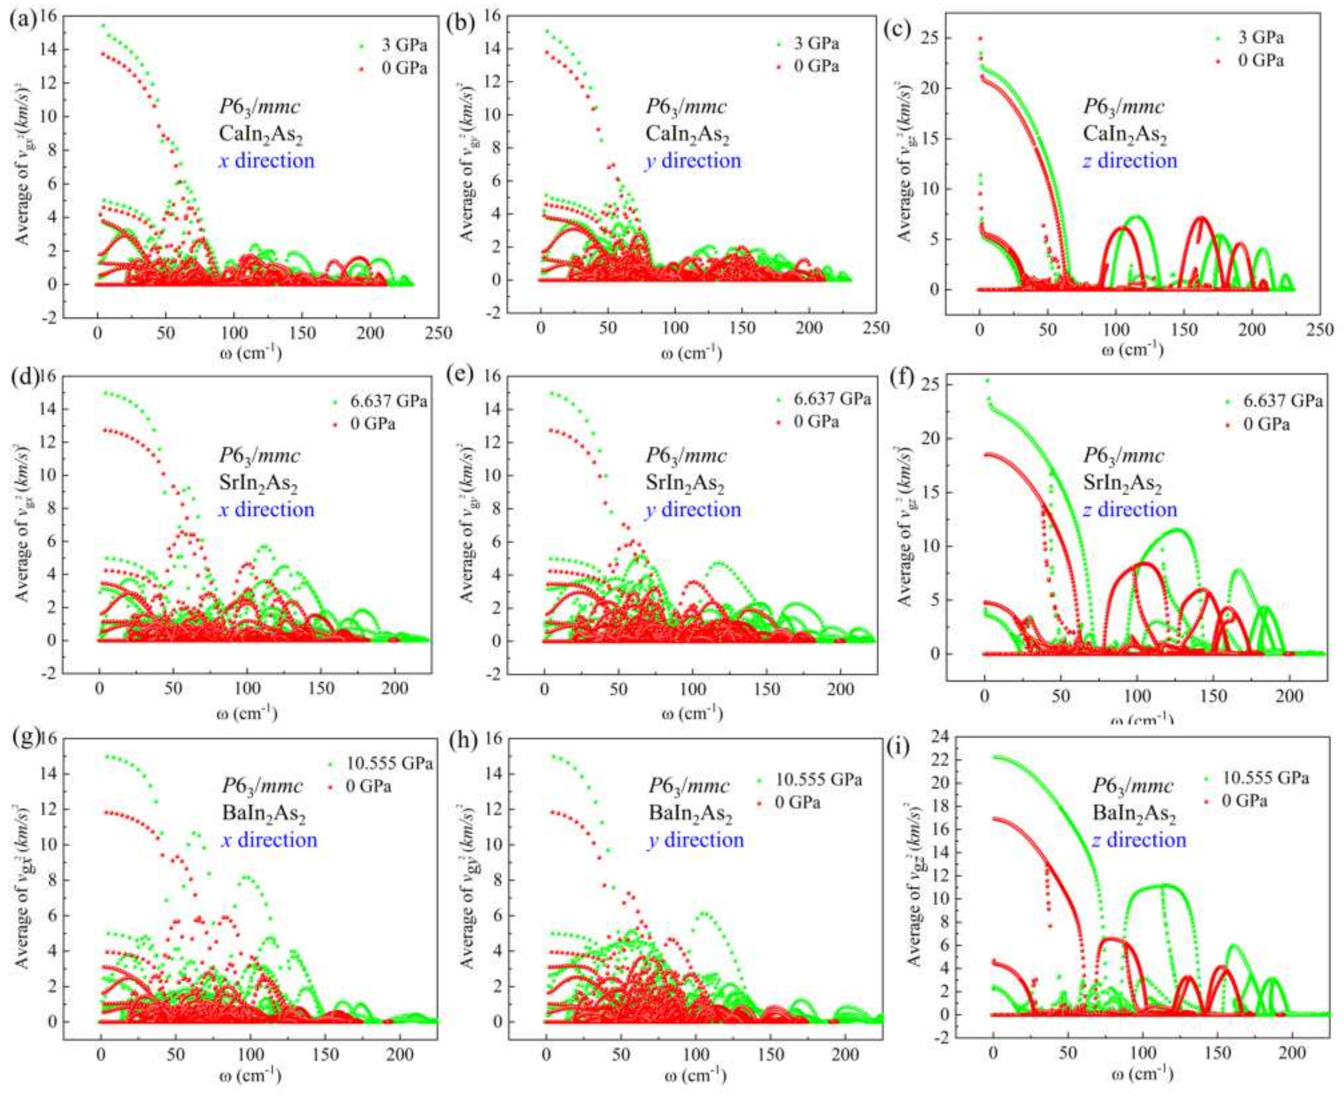


FIG. S18. Projected ($x, y, z$ directions) group velocity distributions dependent on phonon frequencies for the $P6_3/mmc$ phase (a)-(c) $CaIn_2As_2$, (d)-(f) $SrIn_2As_2$, (g)-(i) $BaIn_2As_2$ under different pressure.

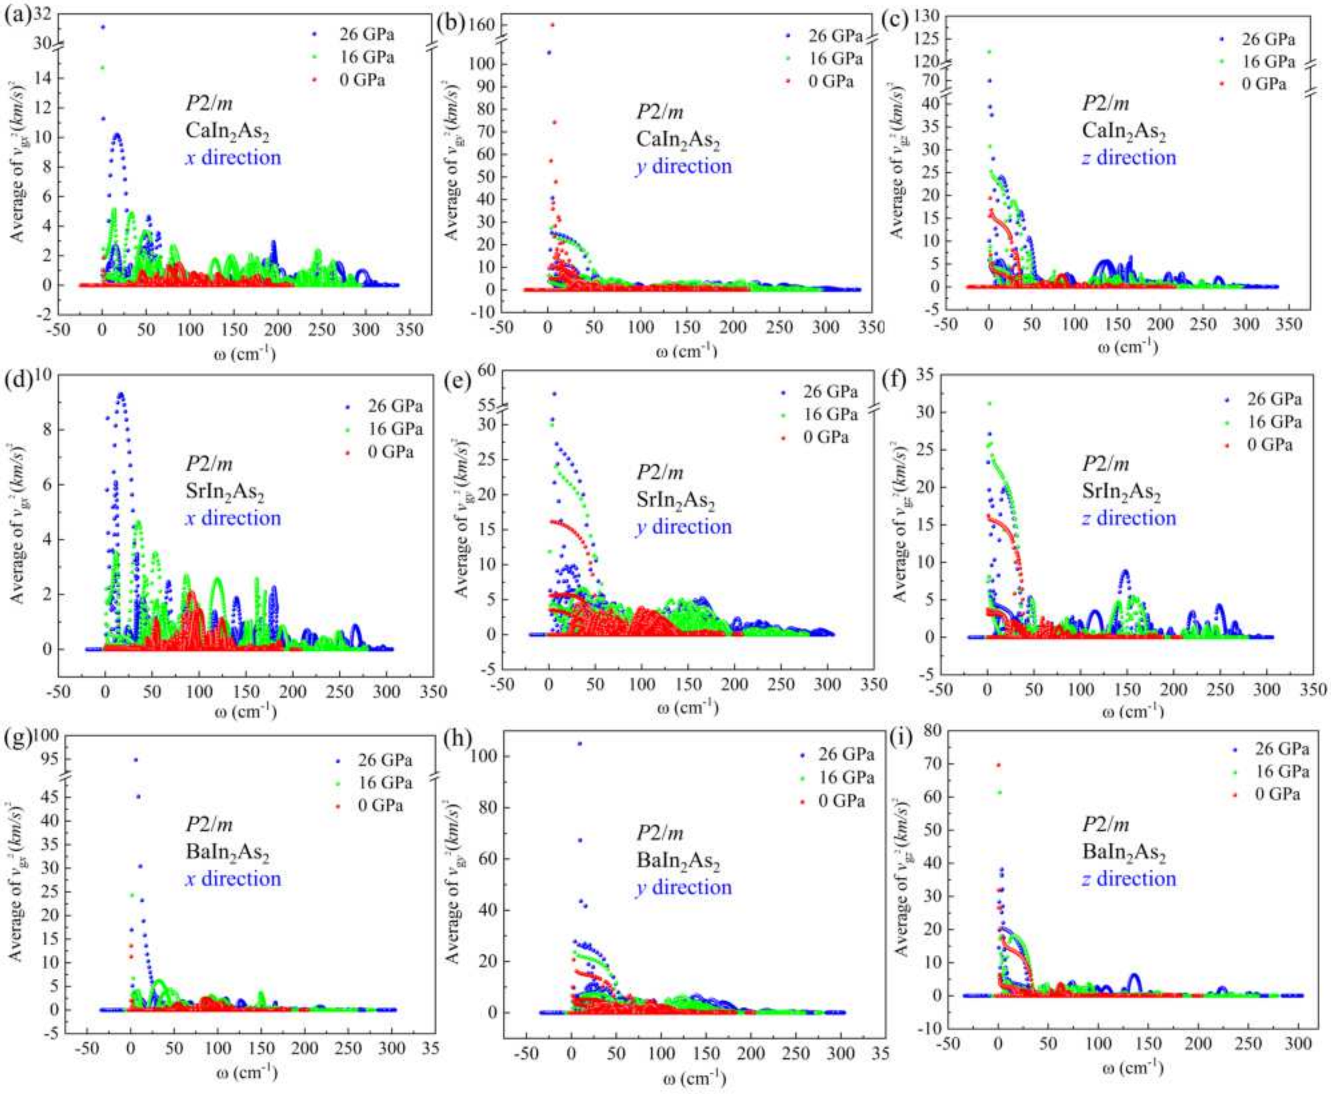


FIG. S19. Projected ($x, y, z$ directions) group velocity distributions dependent on phonon frequencies for the *P*2/*m* phase (a)-(c) $CaIn_2As_2$, (d)-(f) $SrIn_2As_2$, (g)-(i) $BaIn_2As_2$ under different pressure.

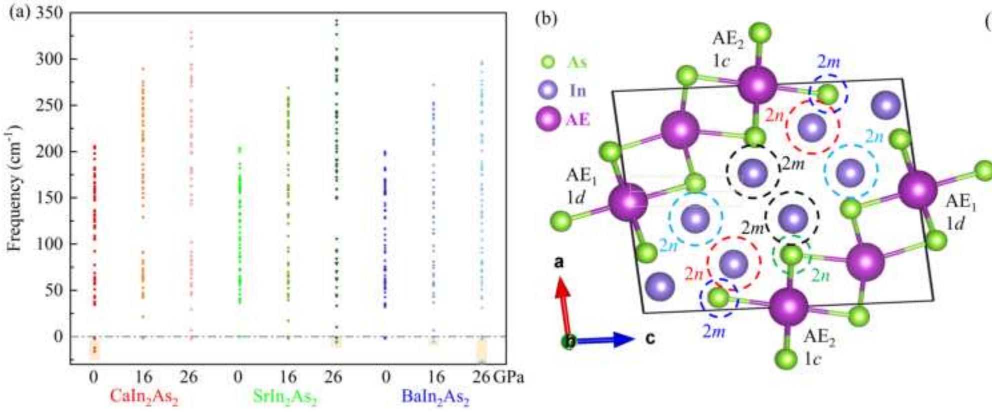


(c)

| System | | Atoms with Wyckoff position |
|---|---|---|
| $CaIn_2As_2$ | 0 GPa | In-2*n*, As-2*m* |
| | 26 GPa | In-2*n*, As-2*m* |
| | | In-2*n*, As-2*n* |
| $SrIn_2As_2$ | 26 GPa | In-2*n*, As-2*m* |
| | | $AE_2$-1*c* |
| $BaIn_2As_2$ | 26 GPa | In-2*m*, As-2*n* |
| | | $AE_1$-1*d*, $AE_2$-1*c* |

FIG. S20. (a) Frequency value distribution of monoclinic phase $AEIn_2As_2$ phonon dispersion spectra at different pressures. (b) Label the atomic sites that are primarily involved in phonon imaginary frequency vibrations. (c) Positions of atoms primarily involved in ZGV contributions at imaginary frequencies.
